# Supplementary material for: The static energy in 2+1+1-flavor QCD
Source: arXiv:2111.02288 source file (2021-11-03)

sm1 - method 2 - 5000 resamples - l3248f211b580m00235m0647m831

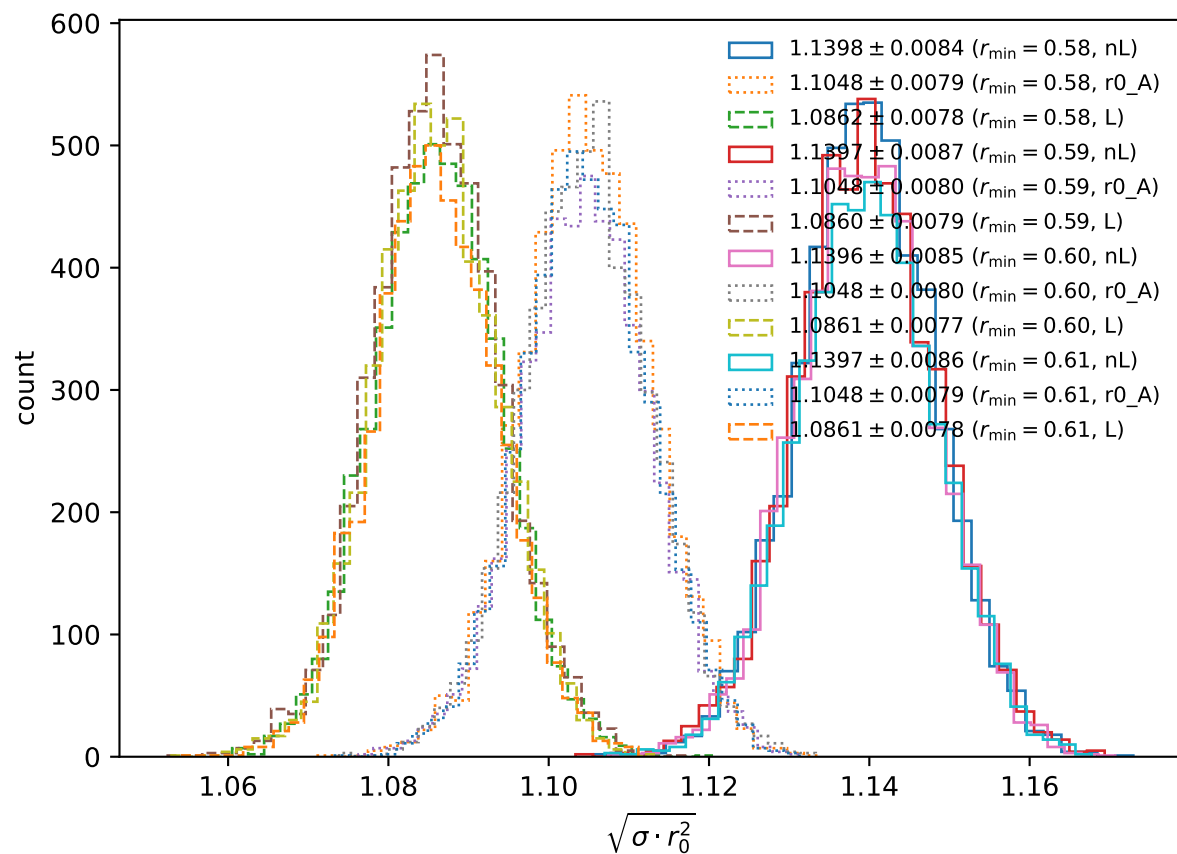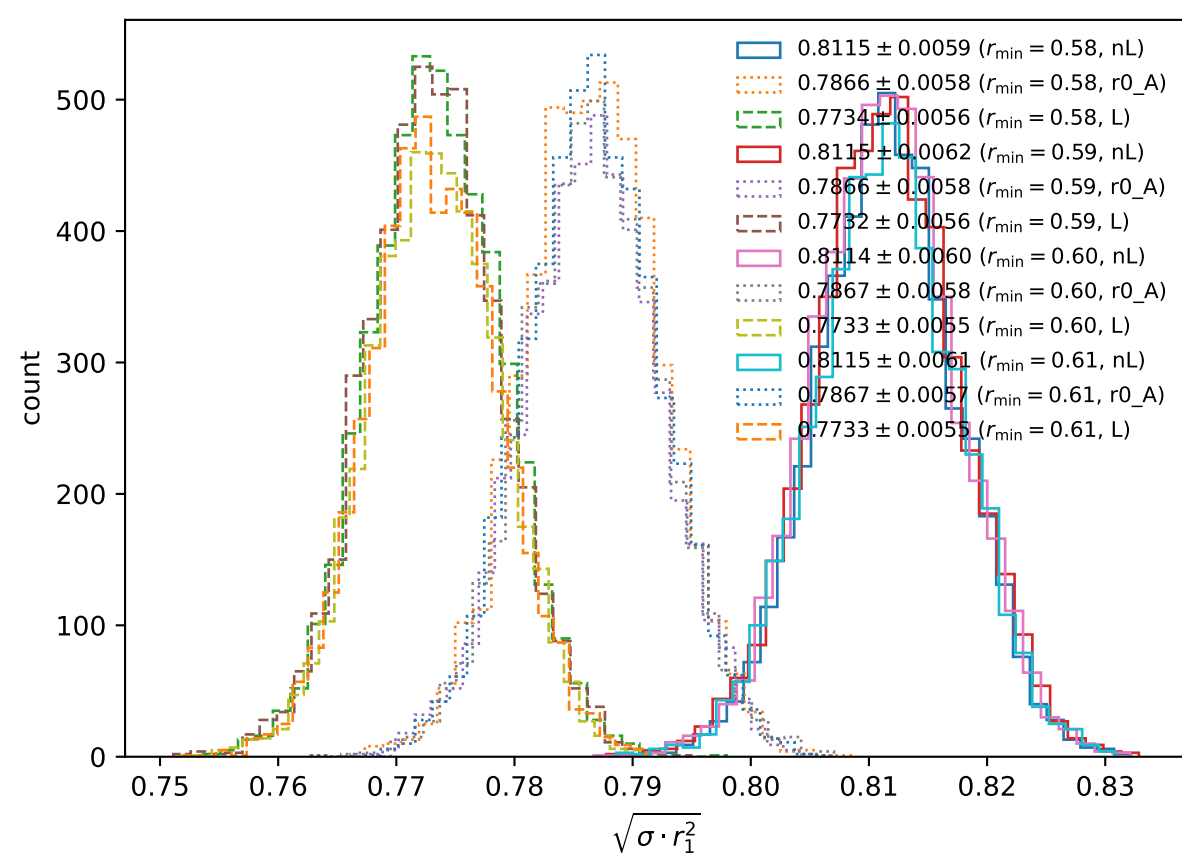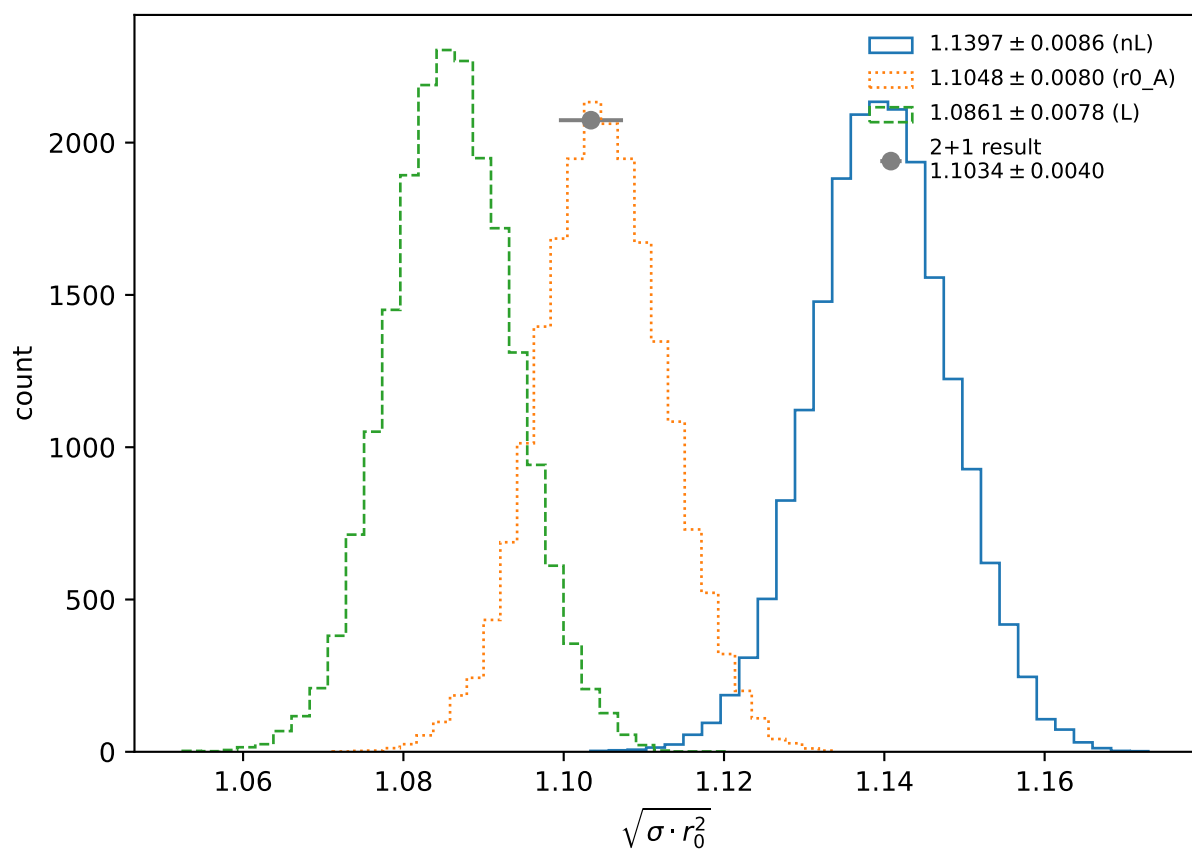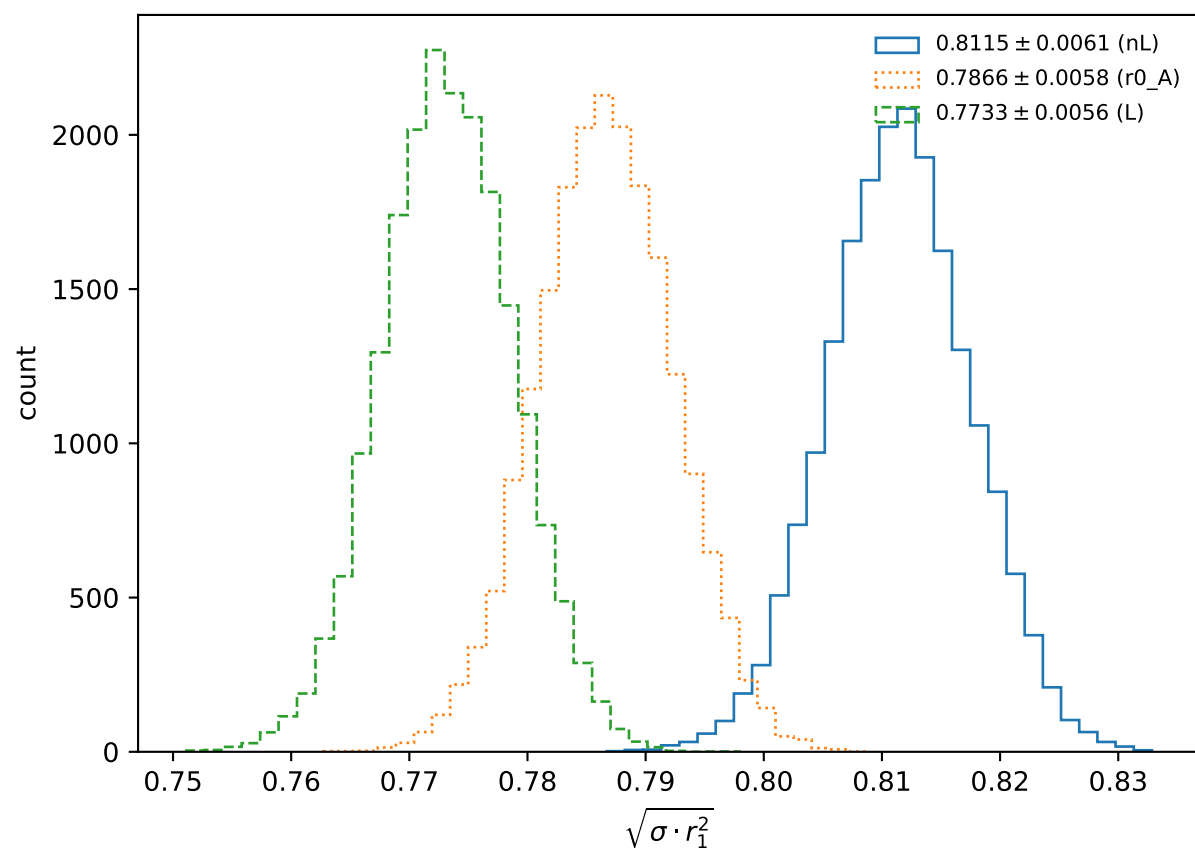

sm1 - method 2 - 5000 resamples - l3264f211b600m00507m0507m628

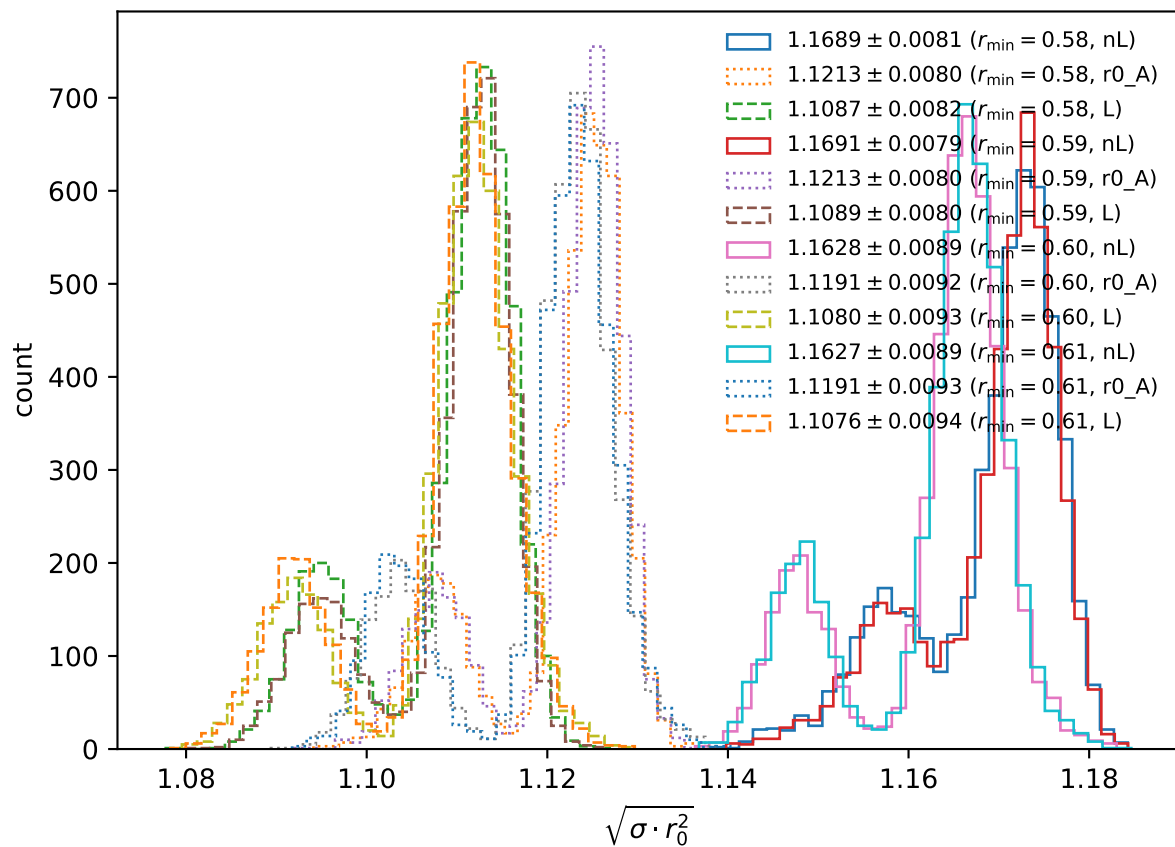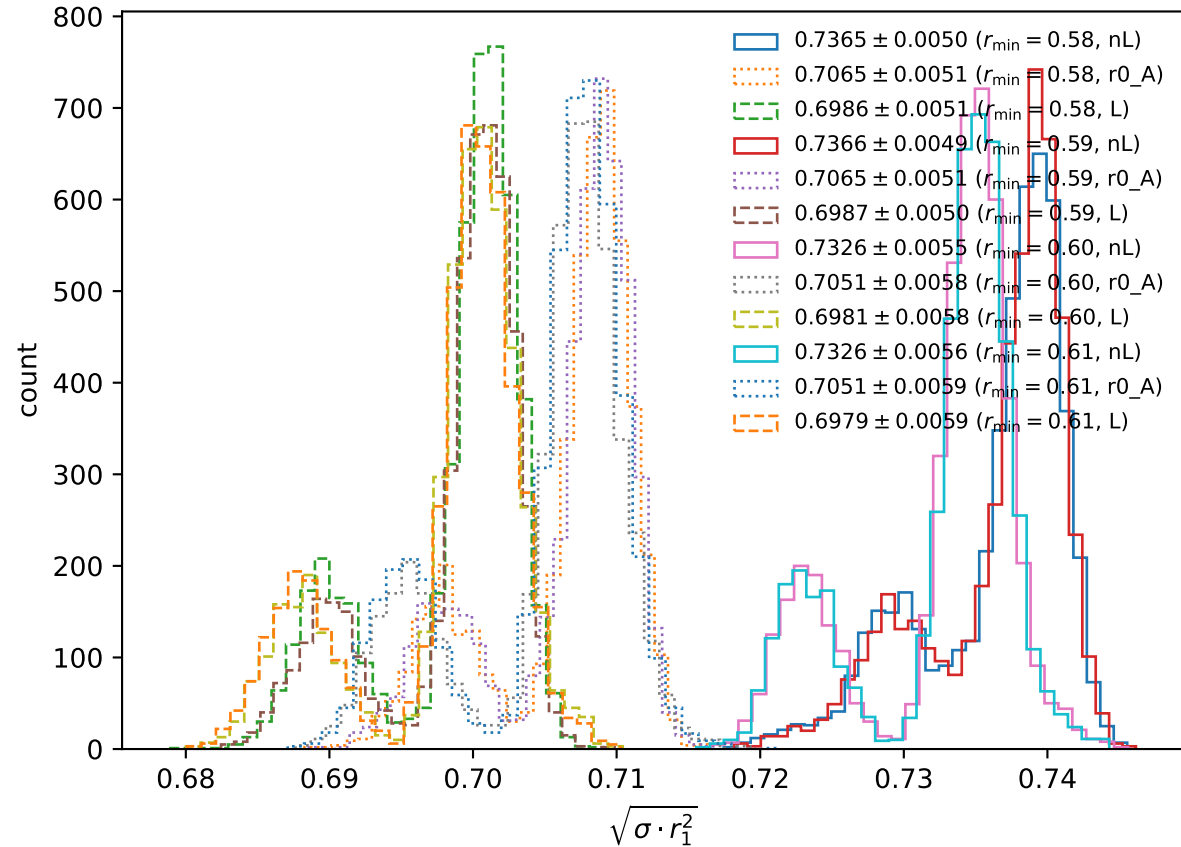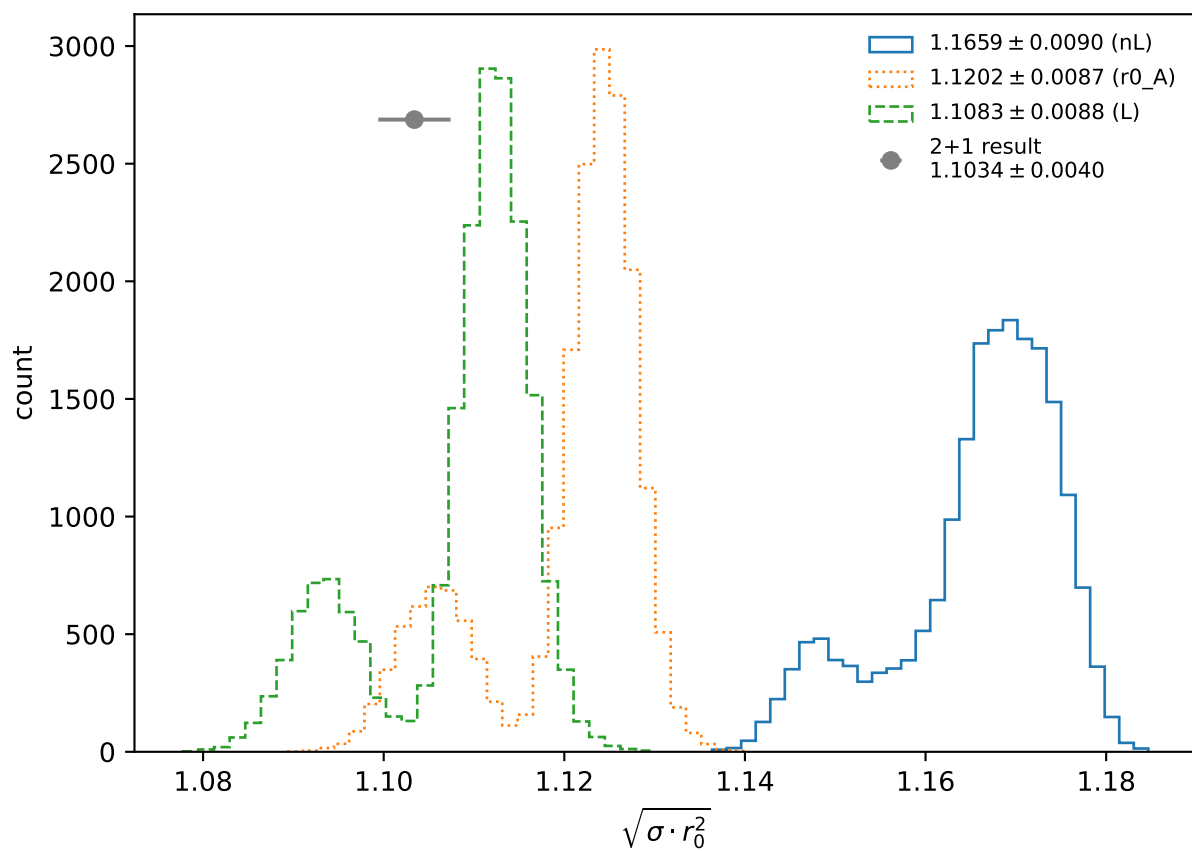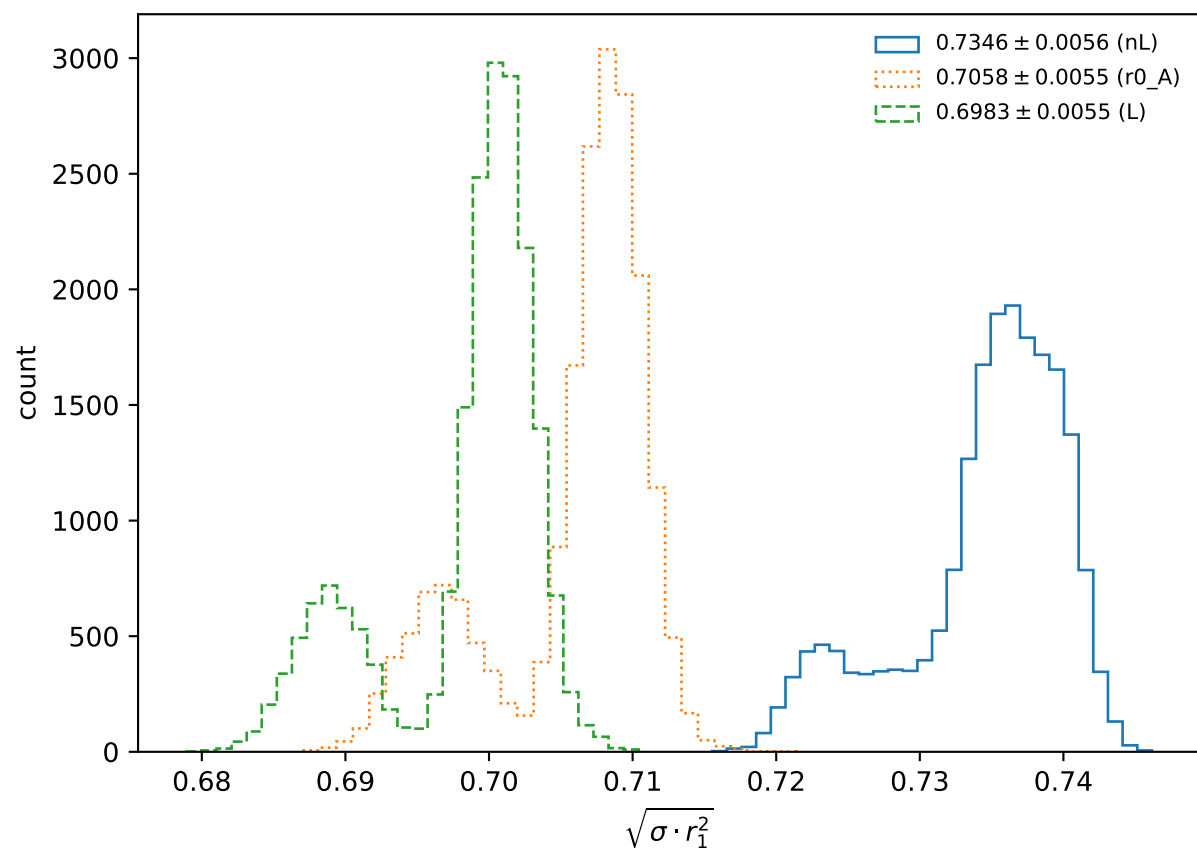

sm1 - method 2 - 5000 resamples - l4864f211b600m00184m0507m628

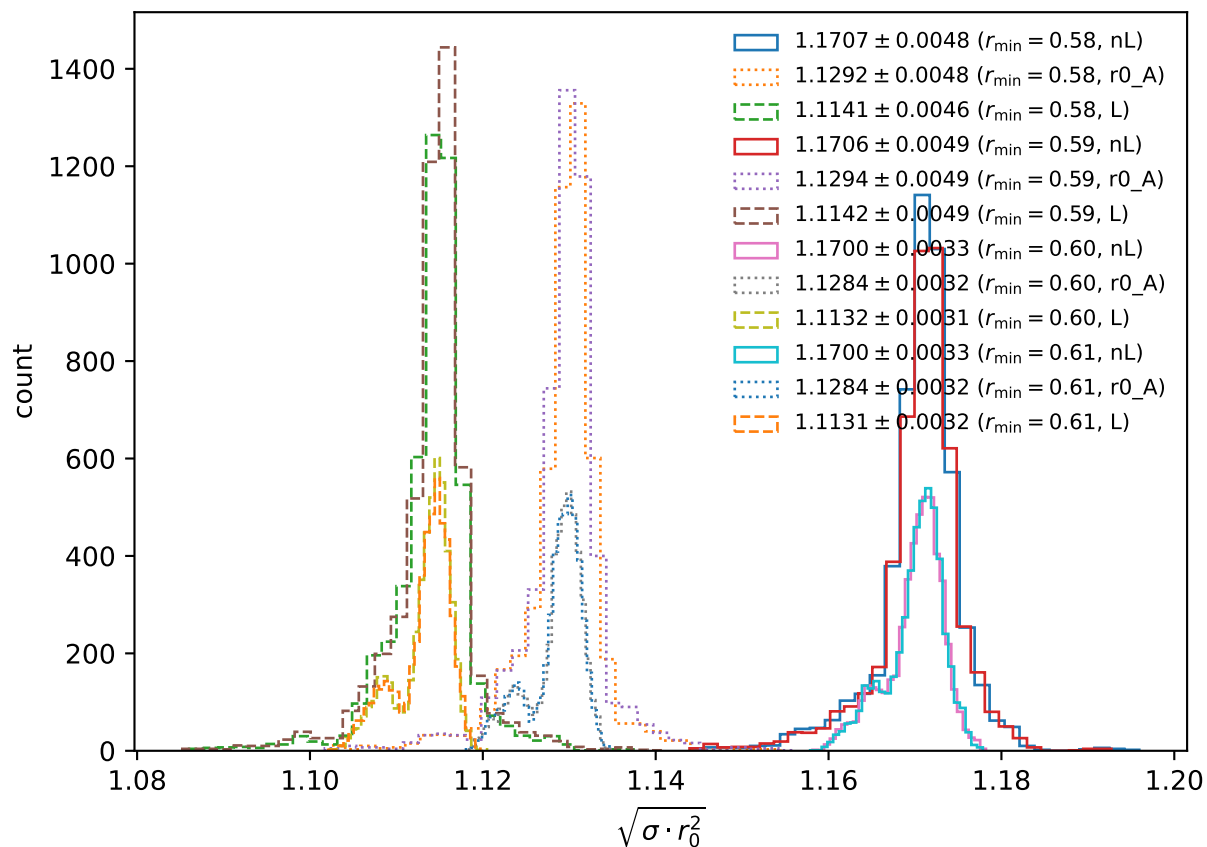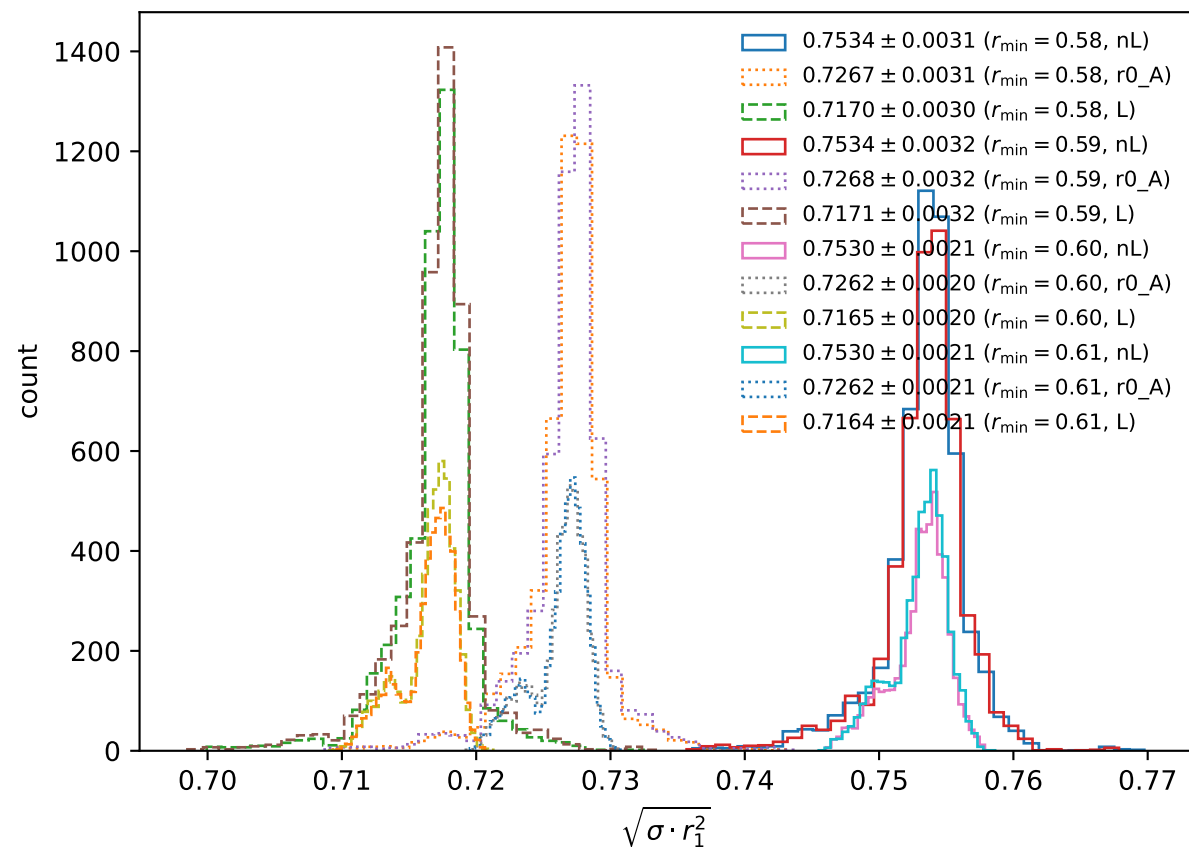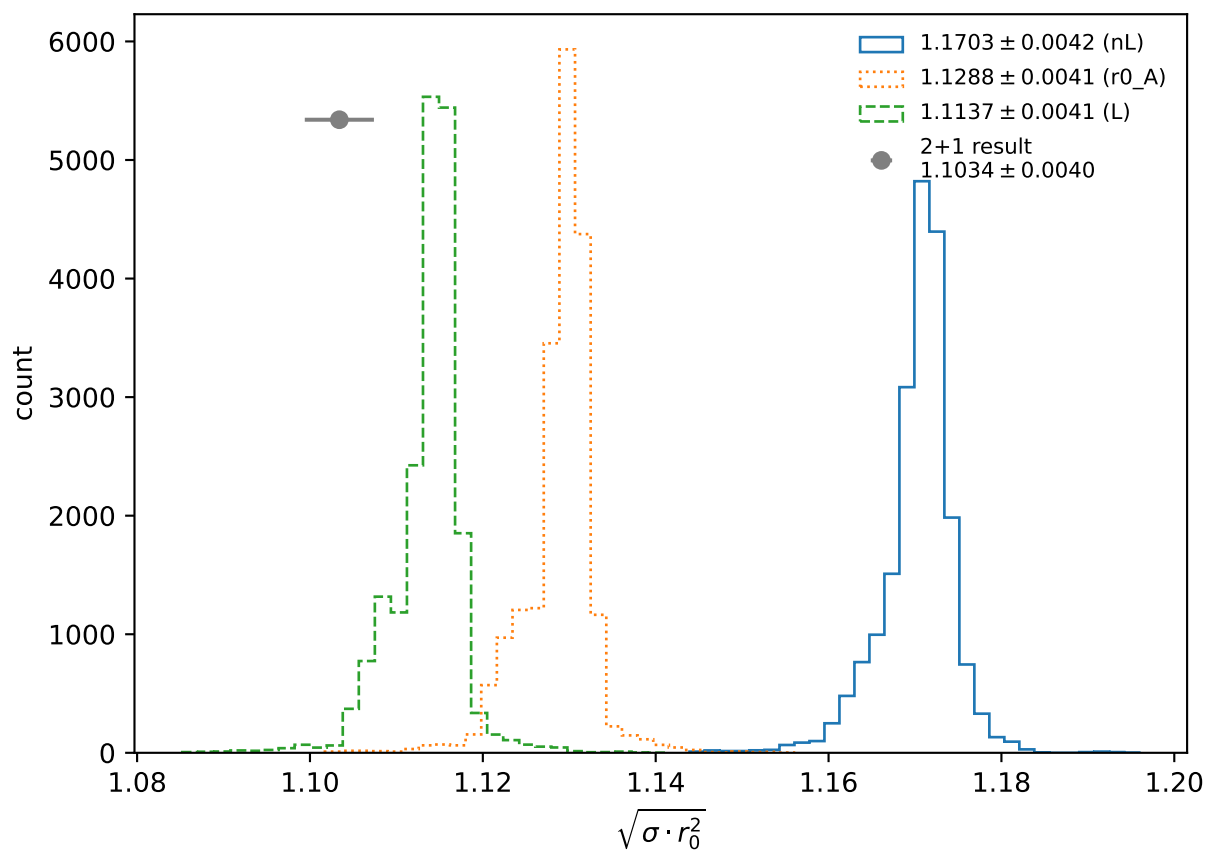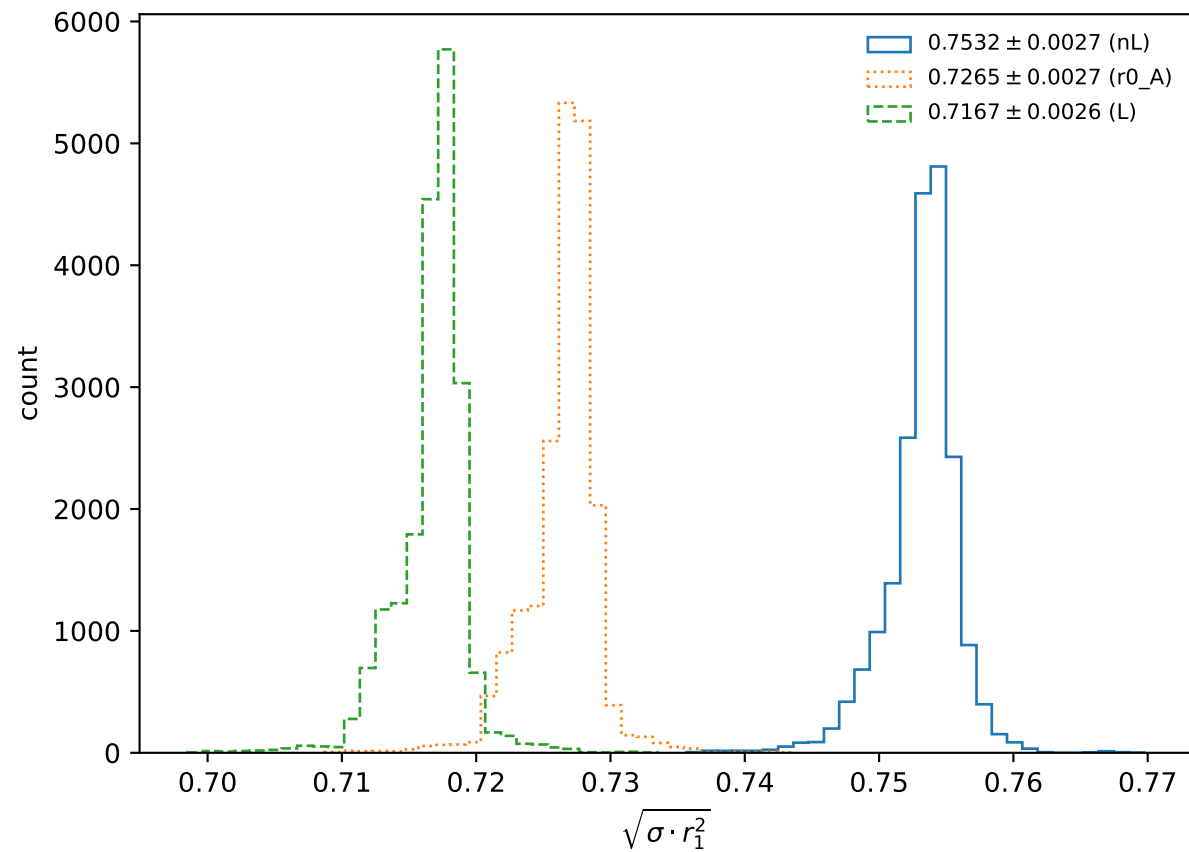

sm1 - method 2 - 5000 resamples - l3296f211b630m0074m037m440

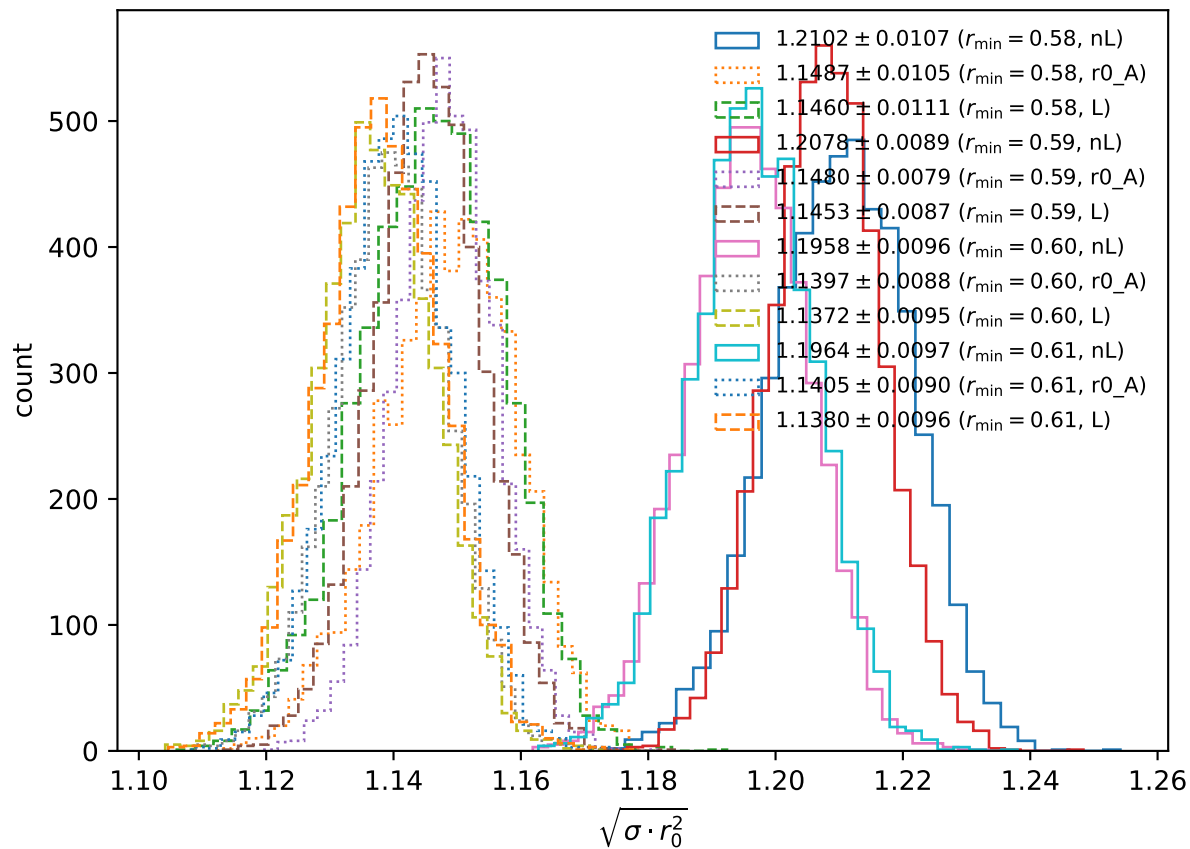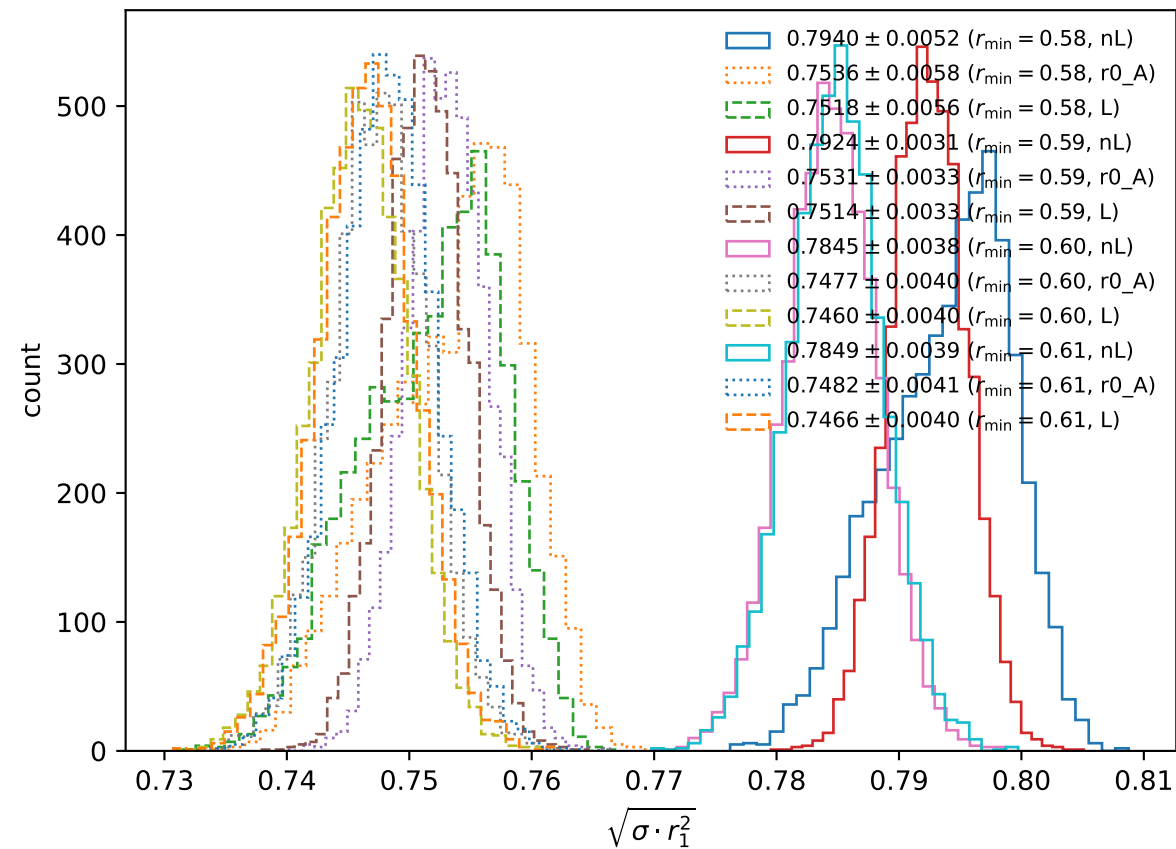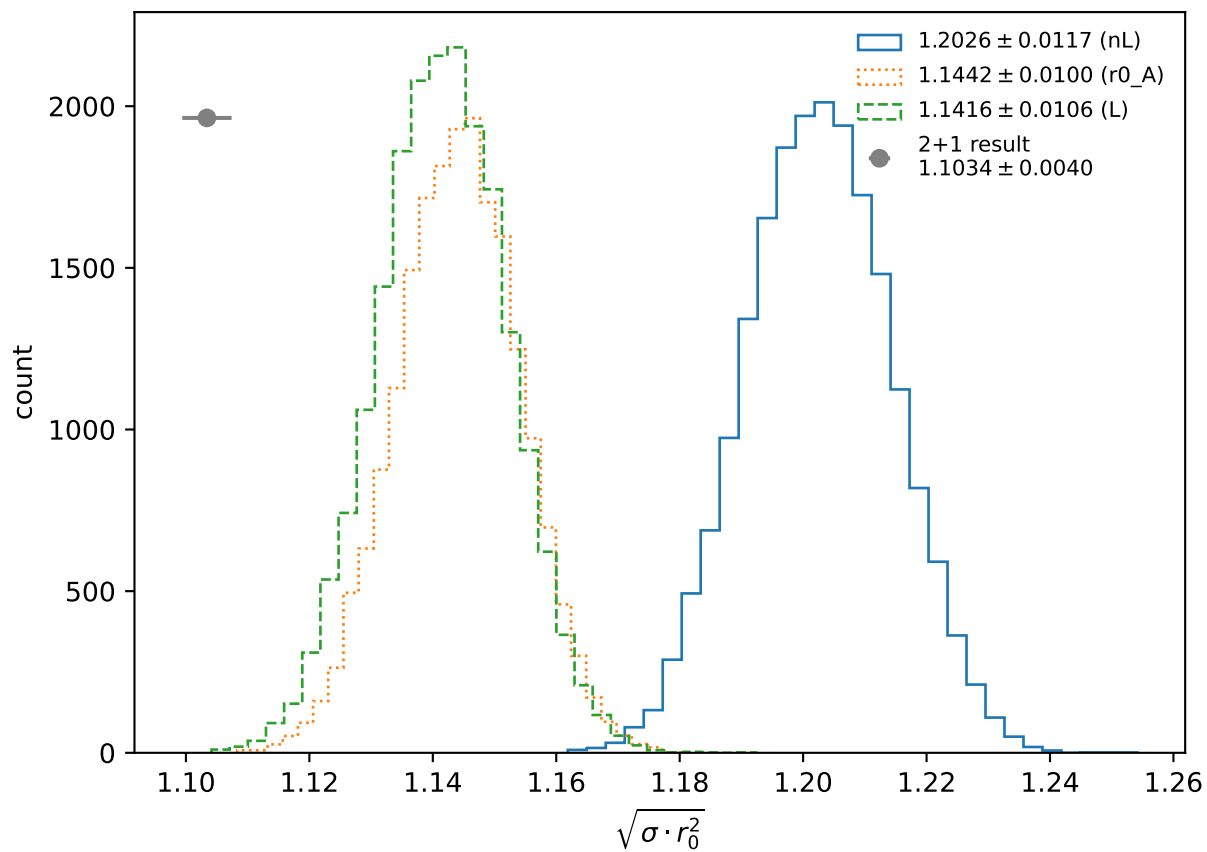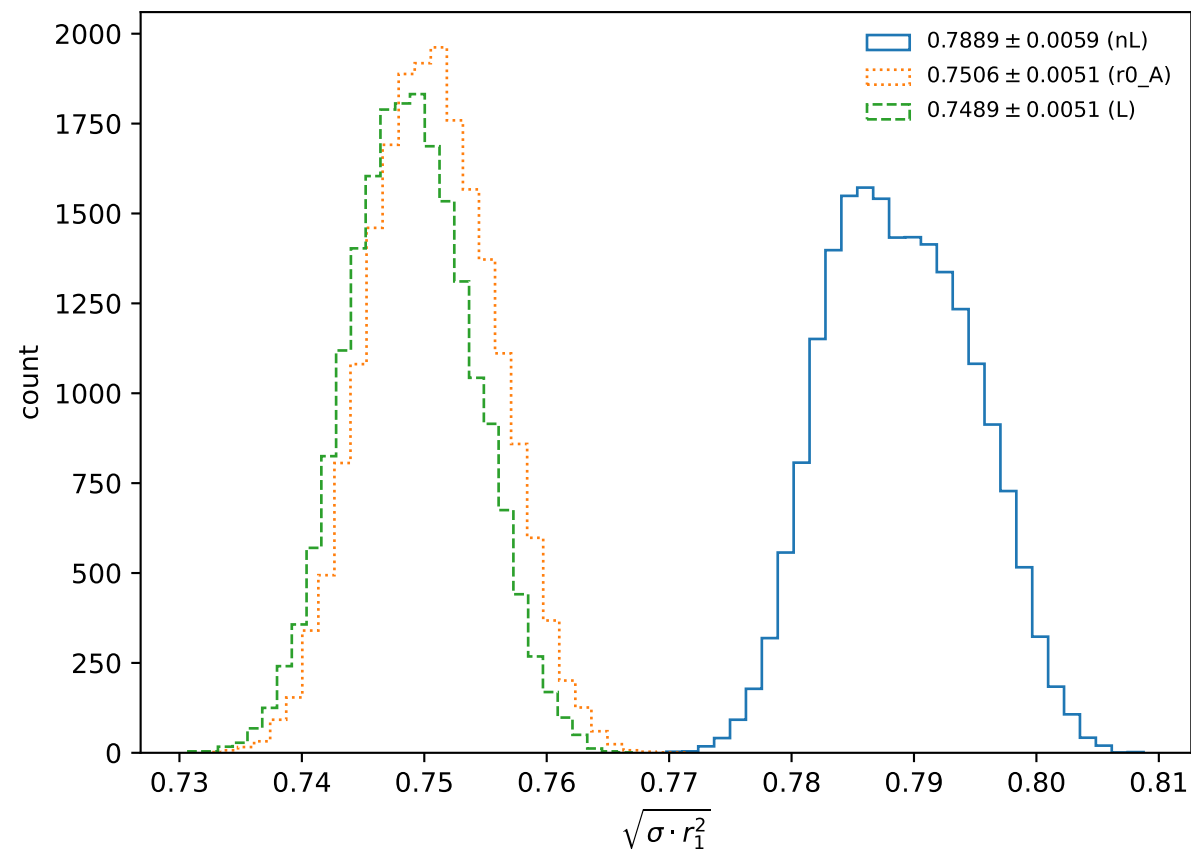

sm1 - method 2 - 5000 resamples - l4896f211b630m00363m0363m430

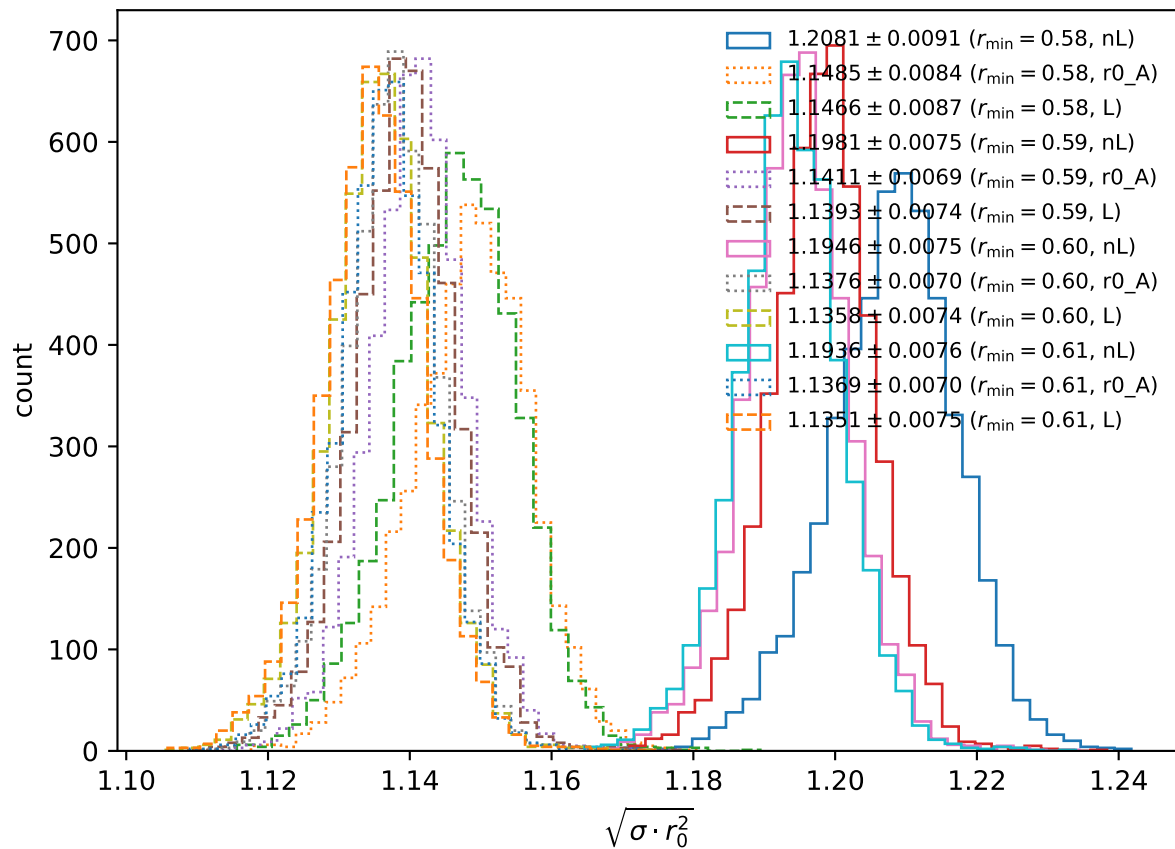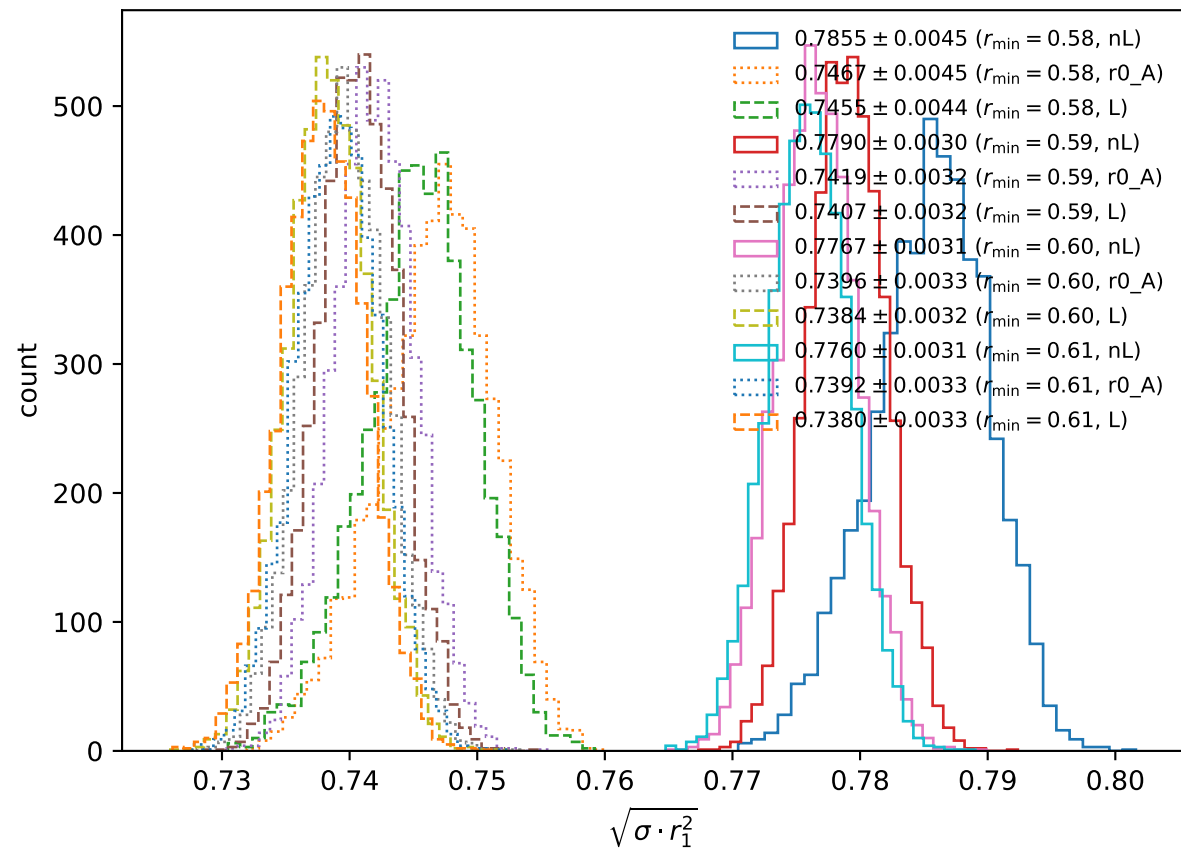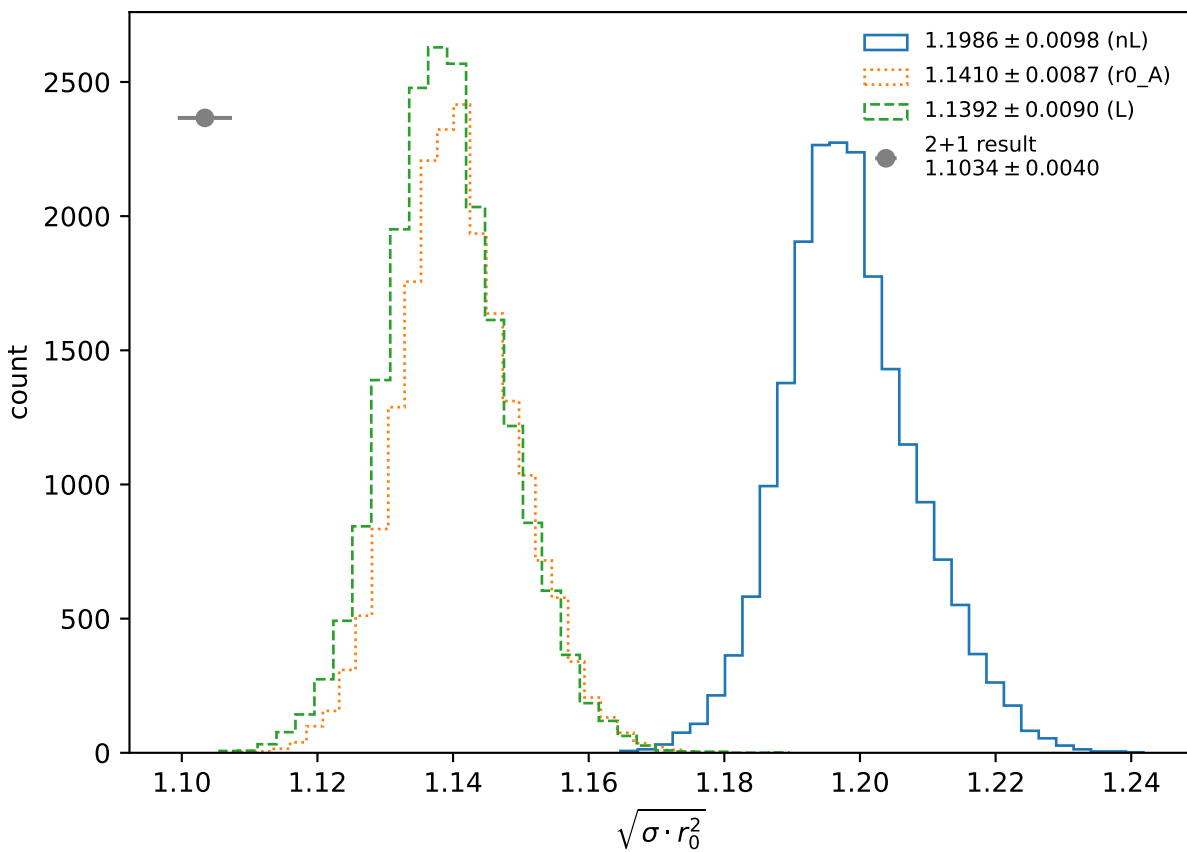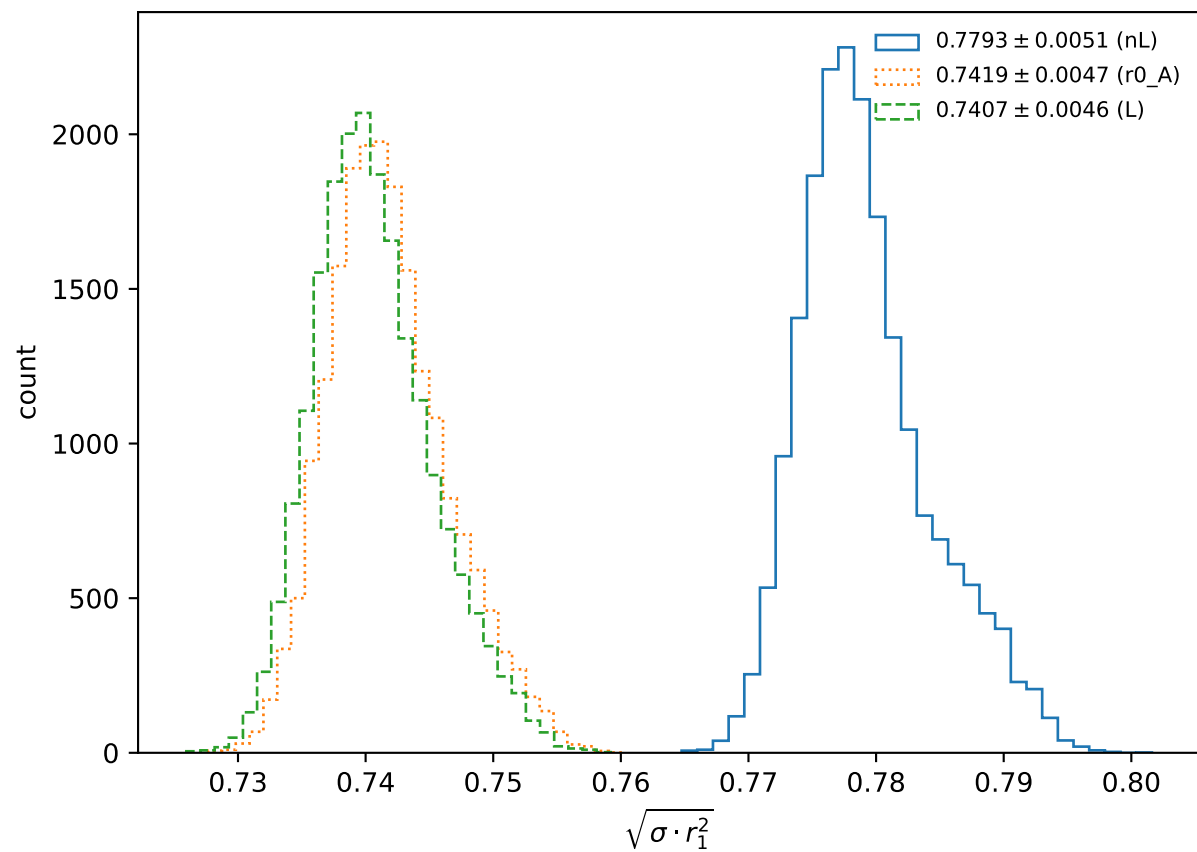

sm1 - method 2 - 5000 resamples - l6496f211b630m0012m0363m432

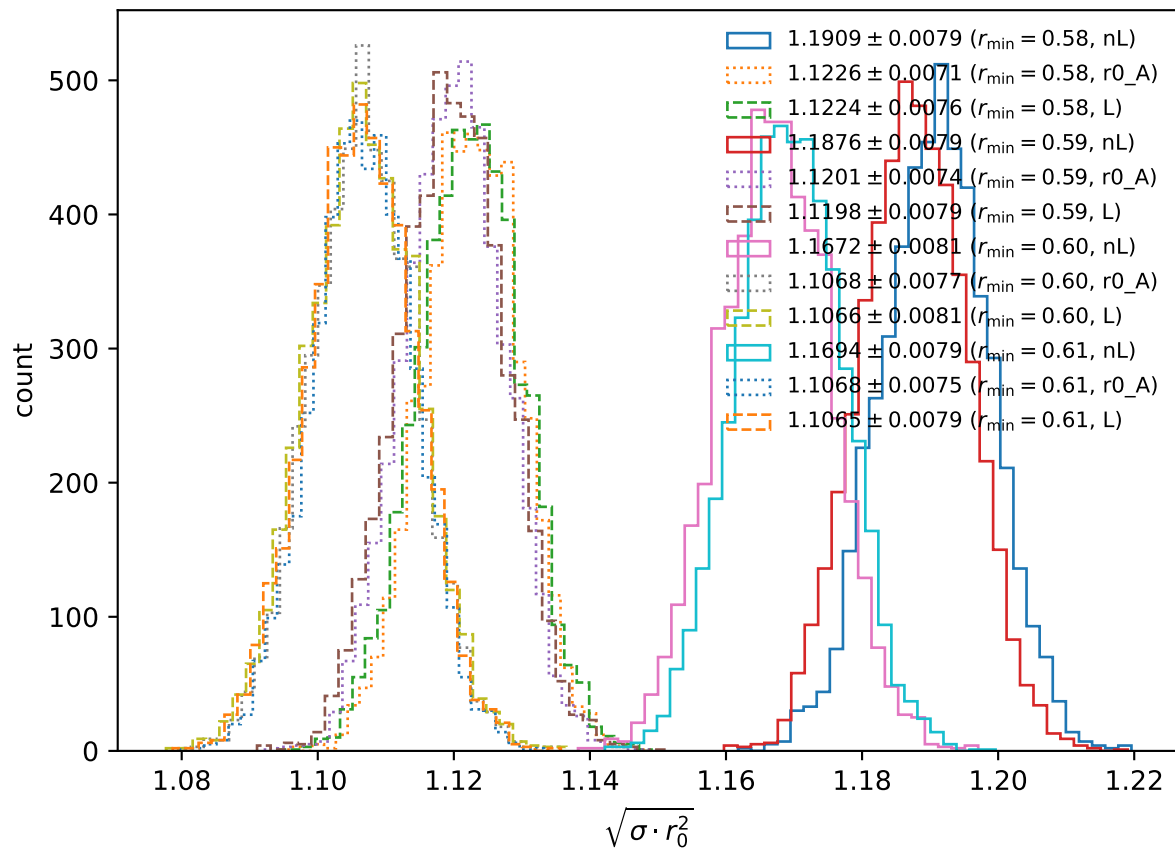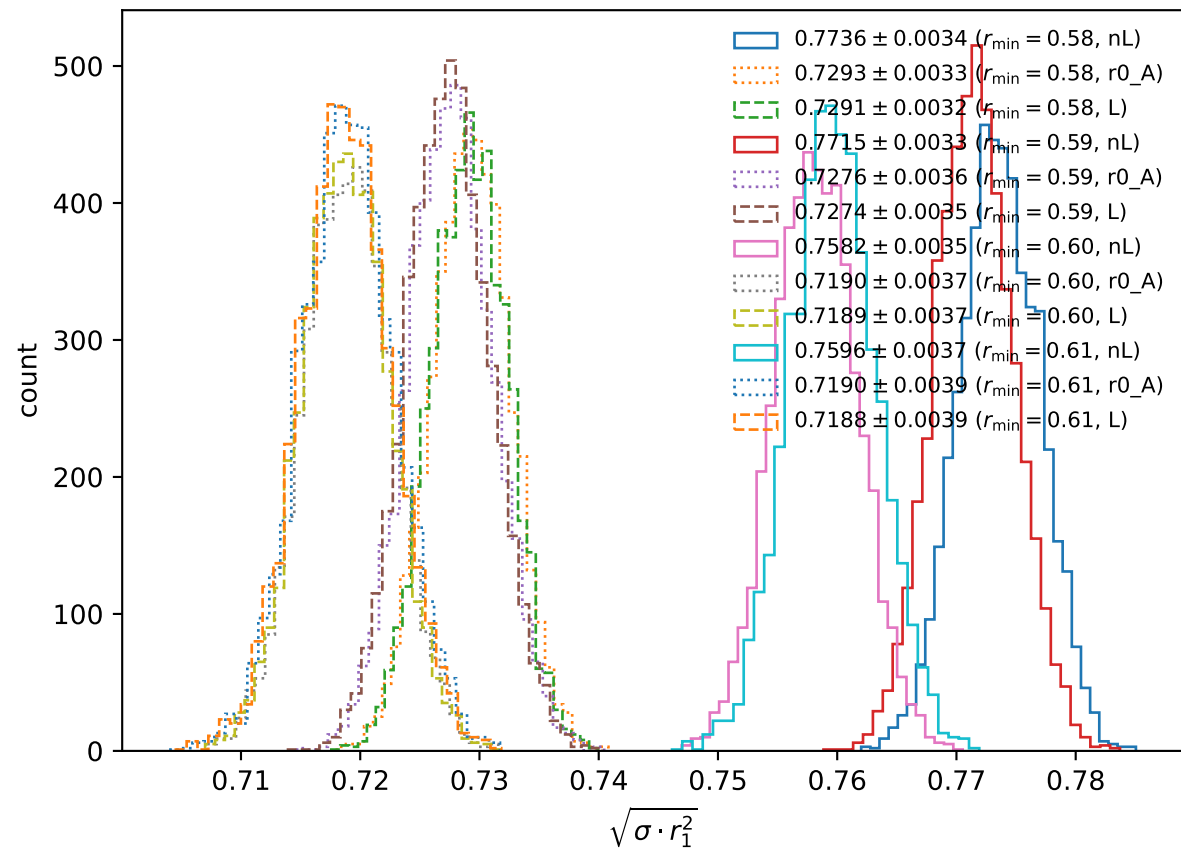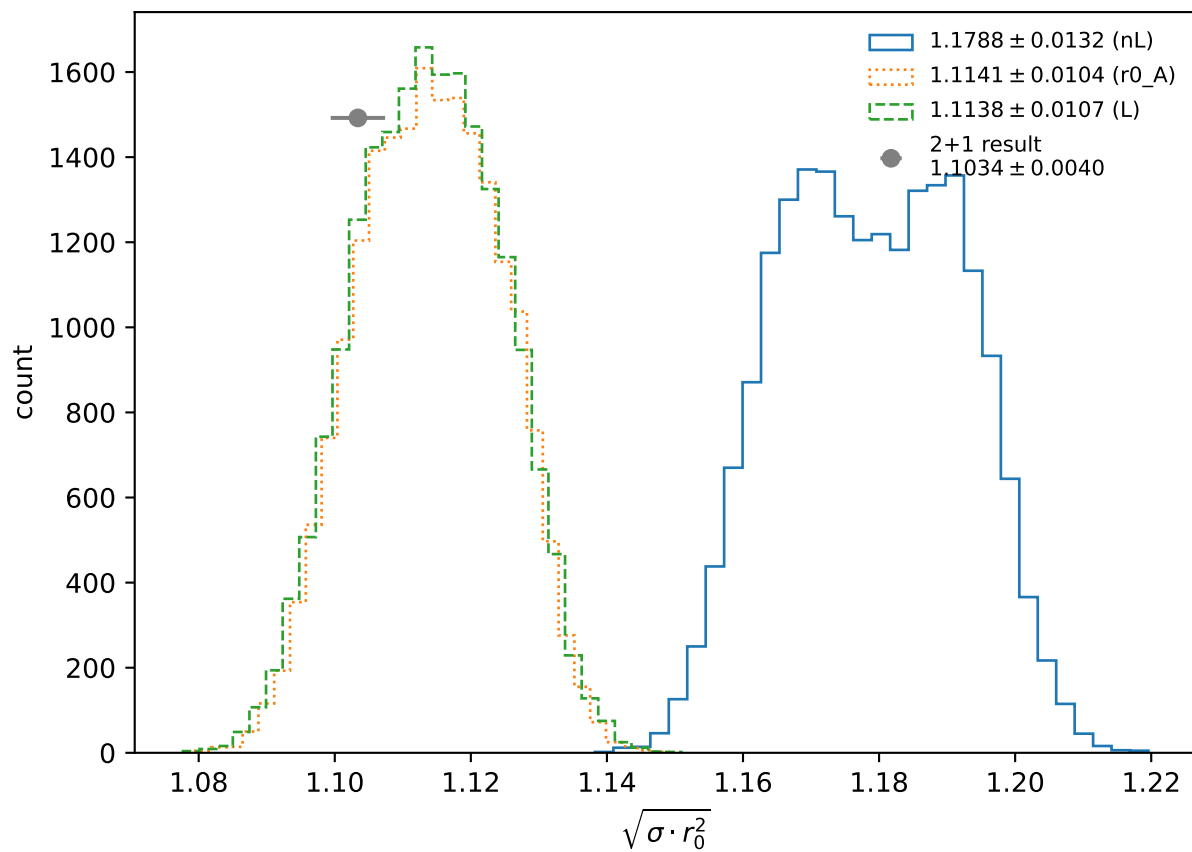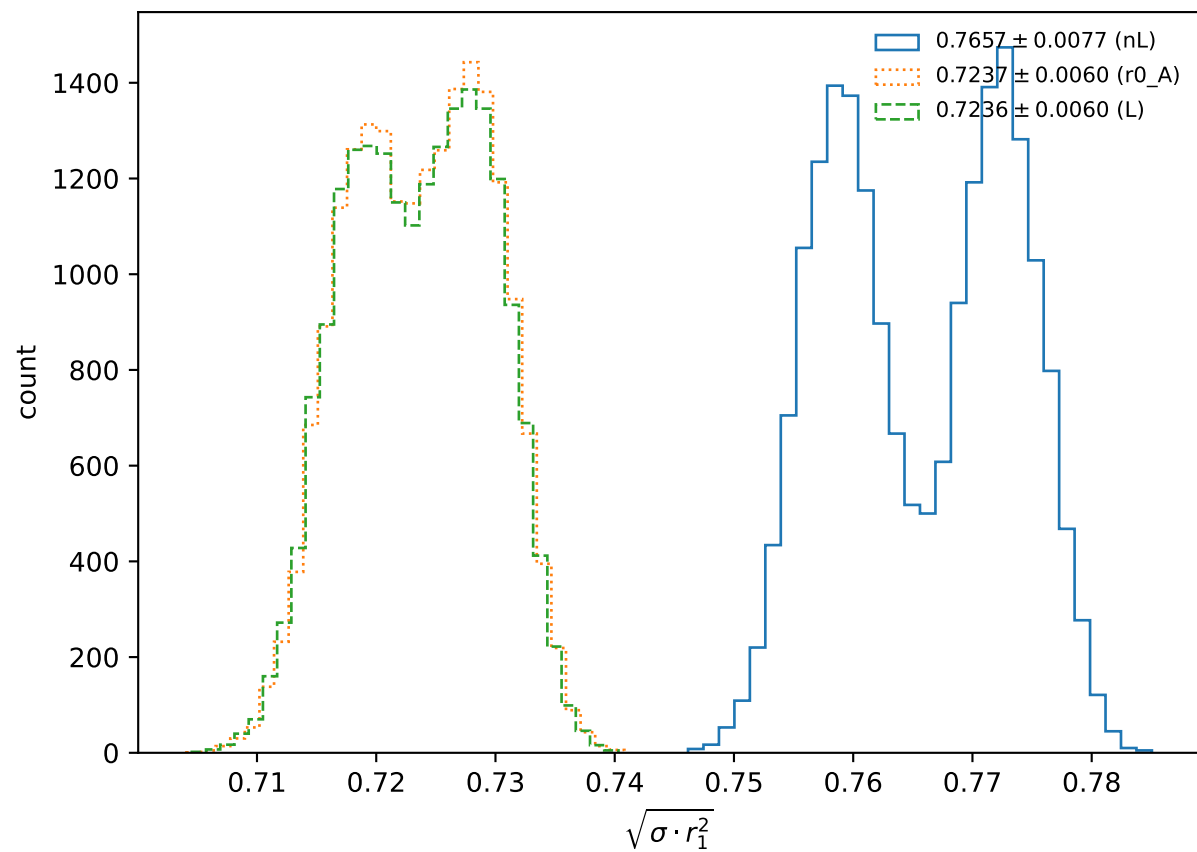

sm1 - method 2 - 5000 resamples - l48144f211b672m0048m024m286

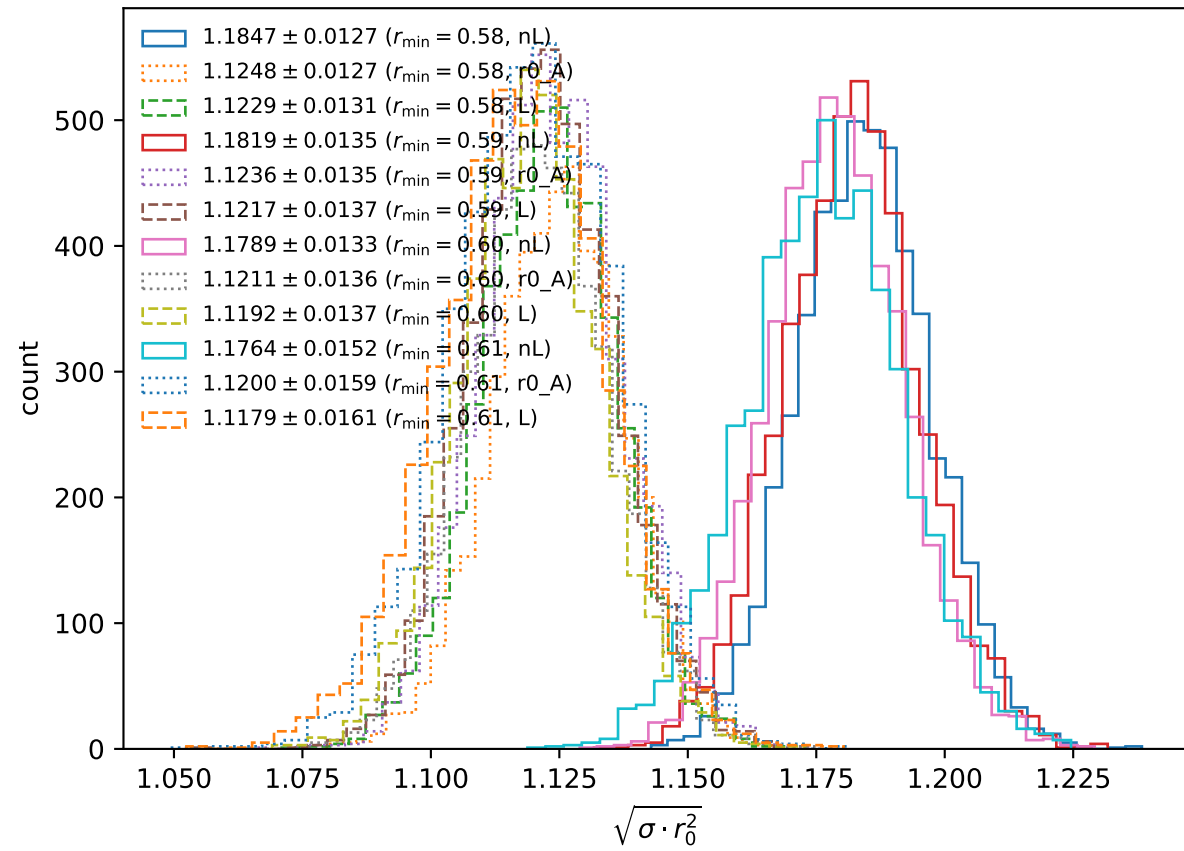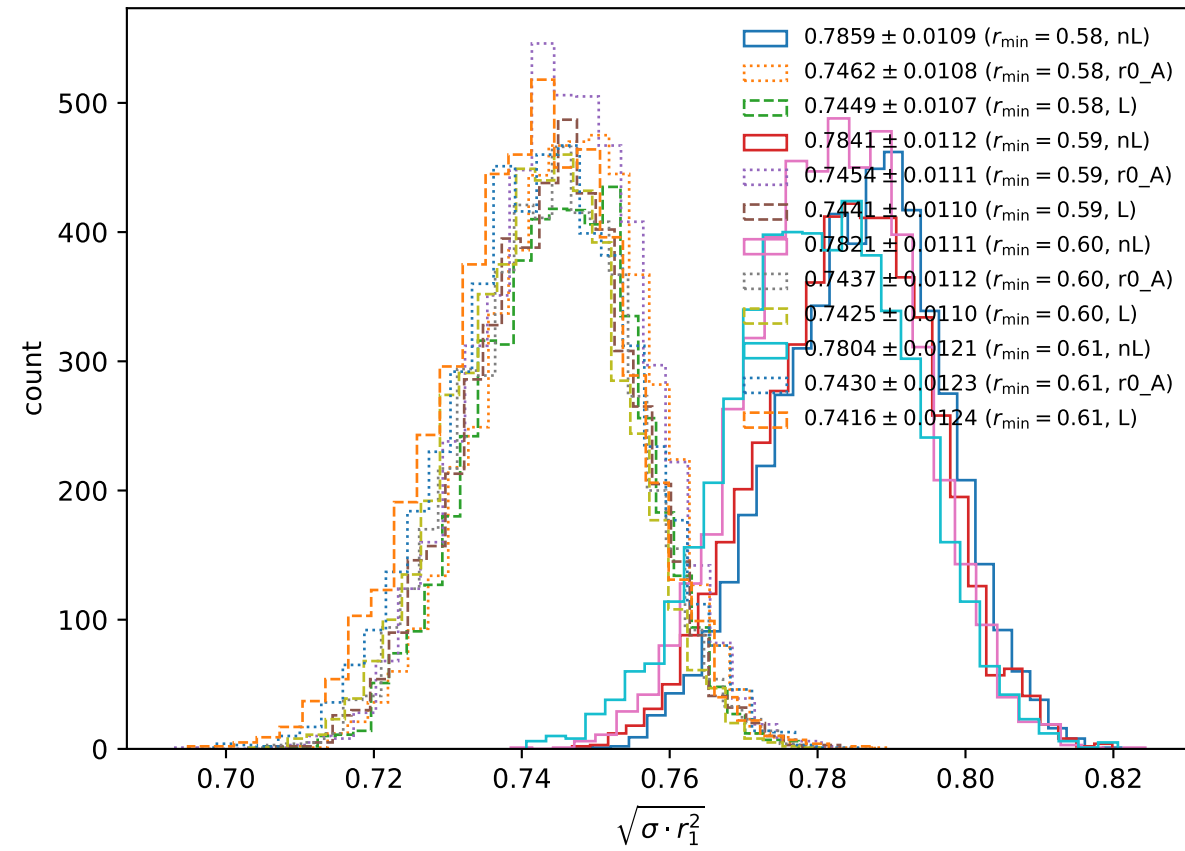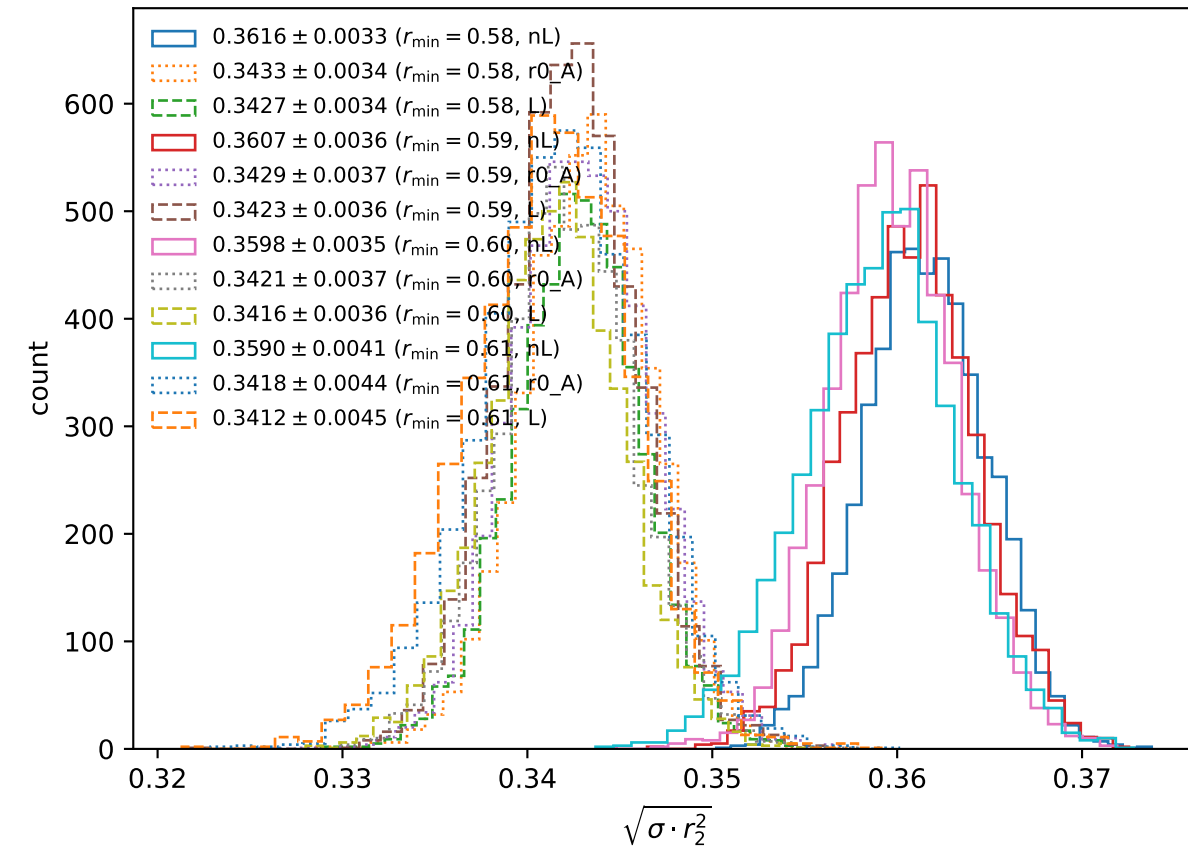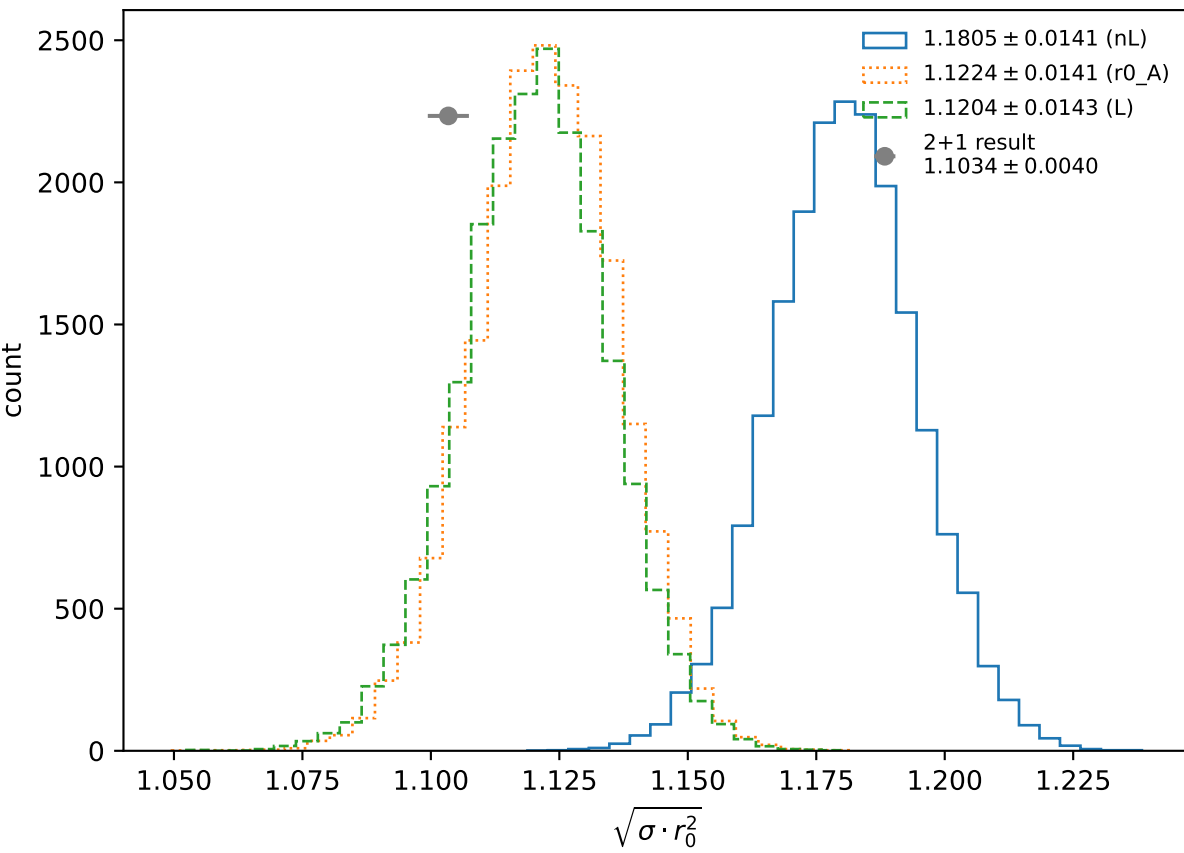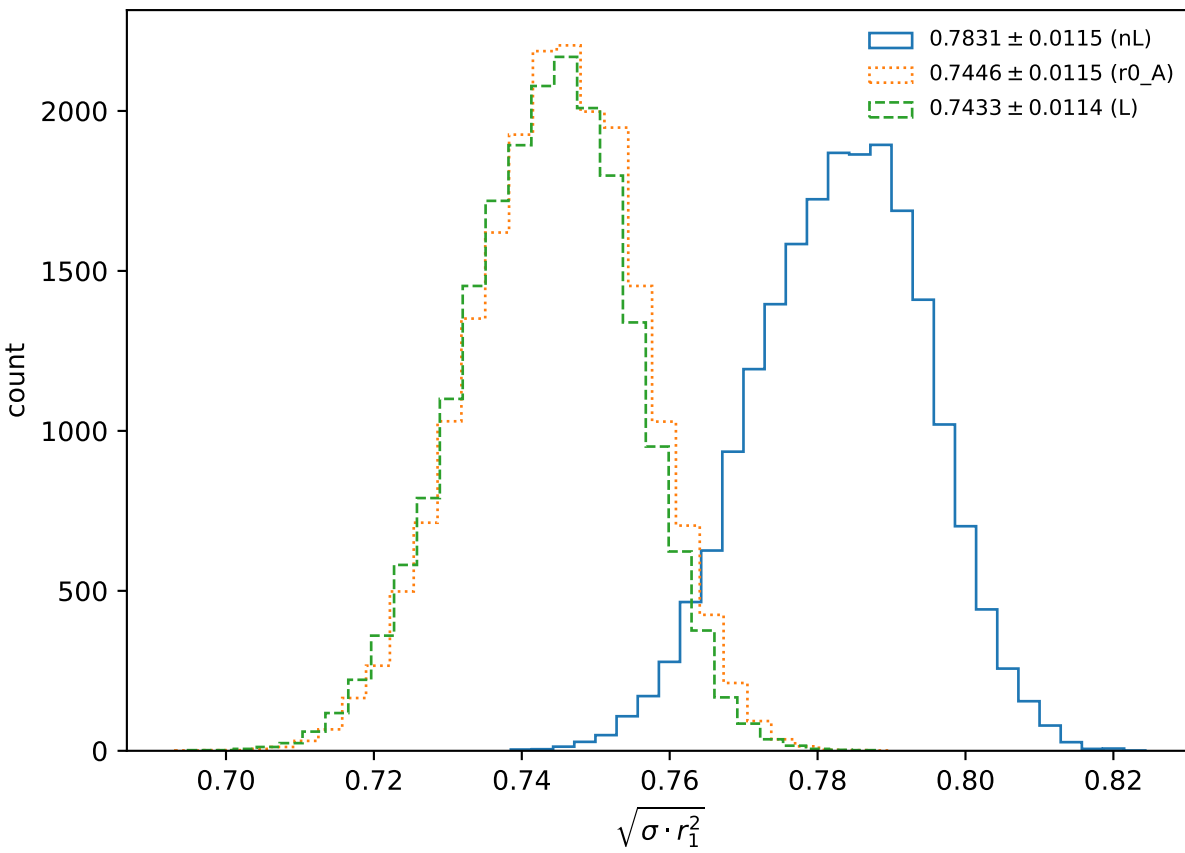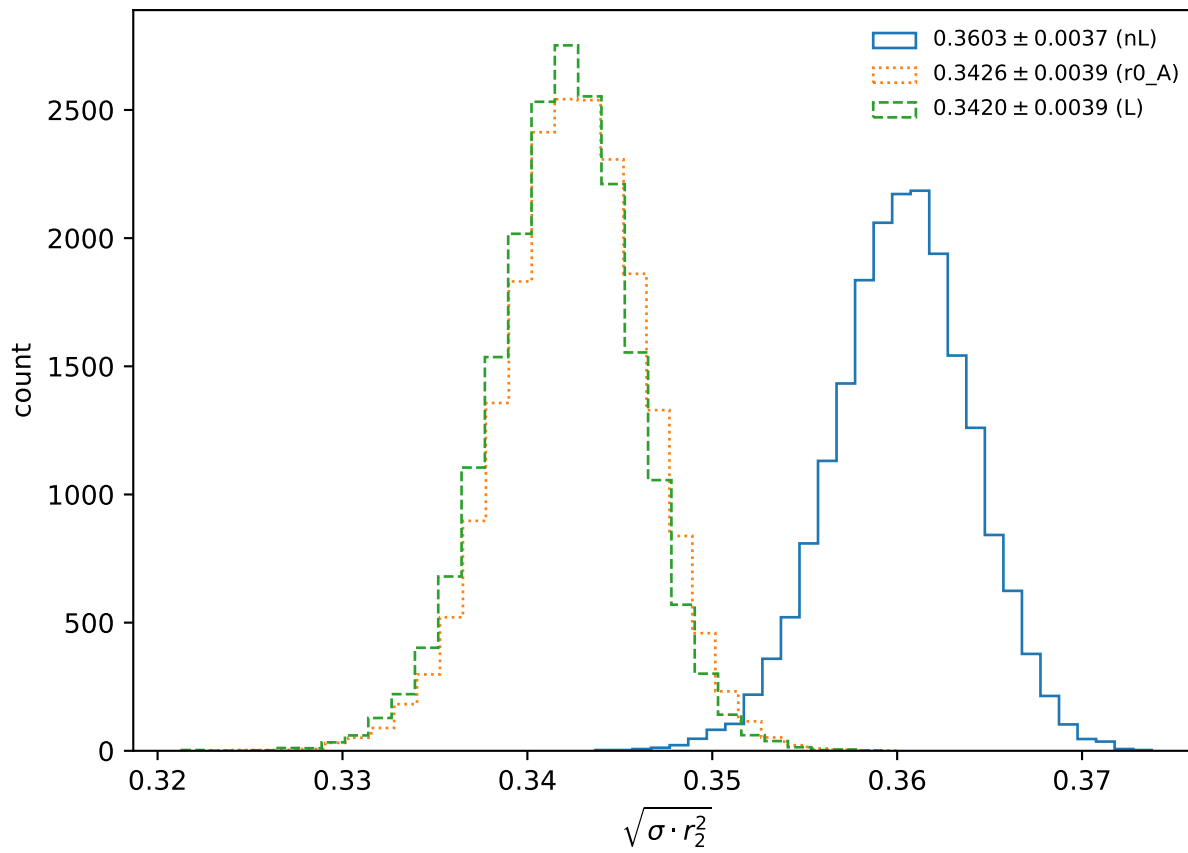



sm1 - method 2 - 5000 resamples - l64144f211b672m0024m024m286

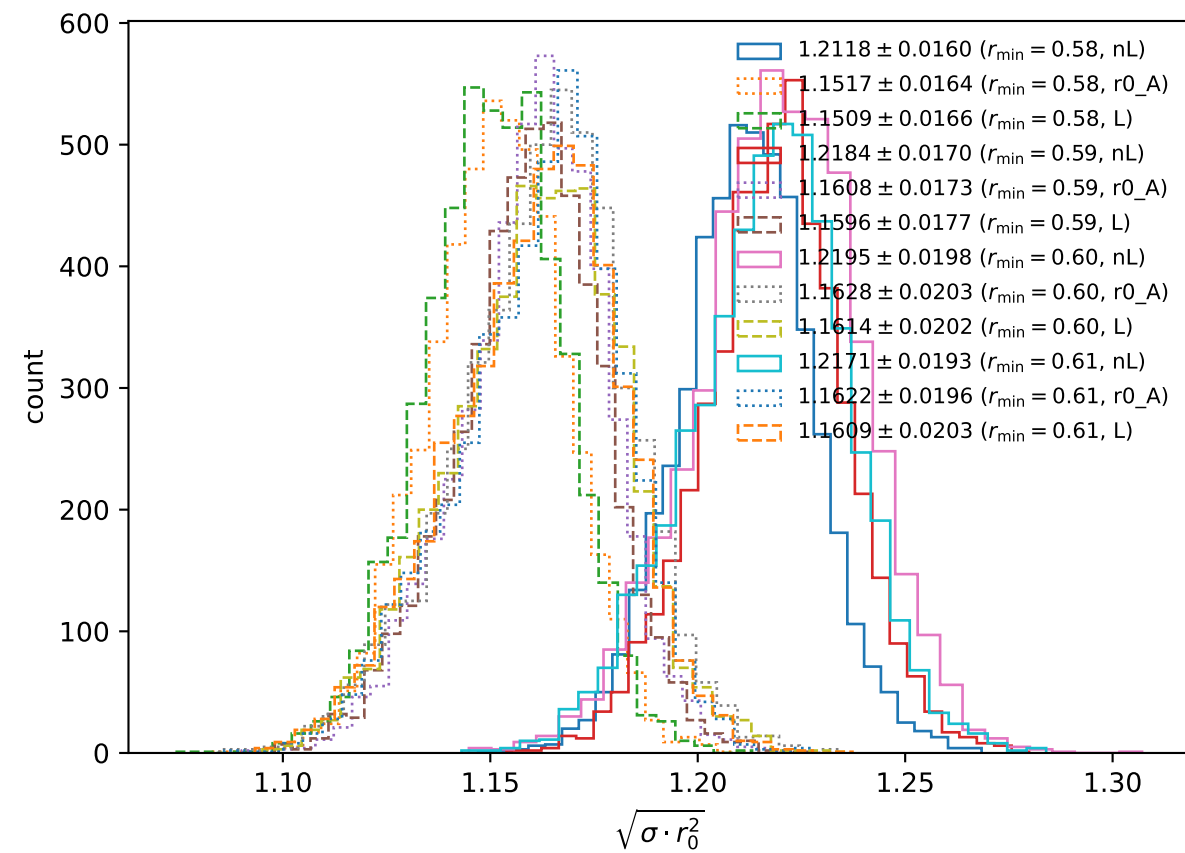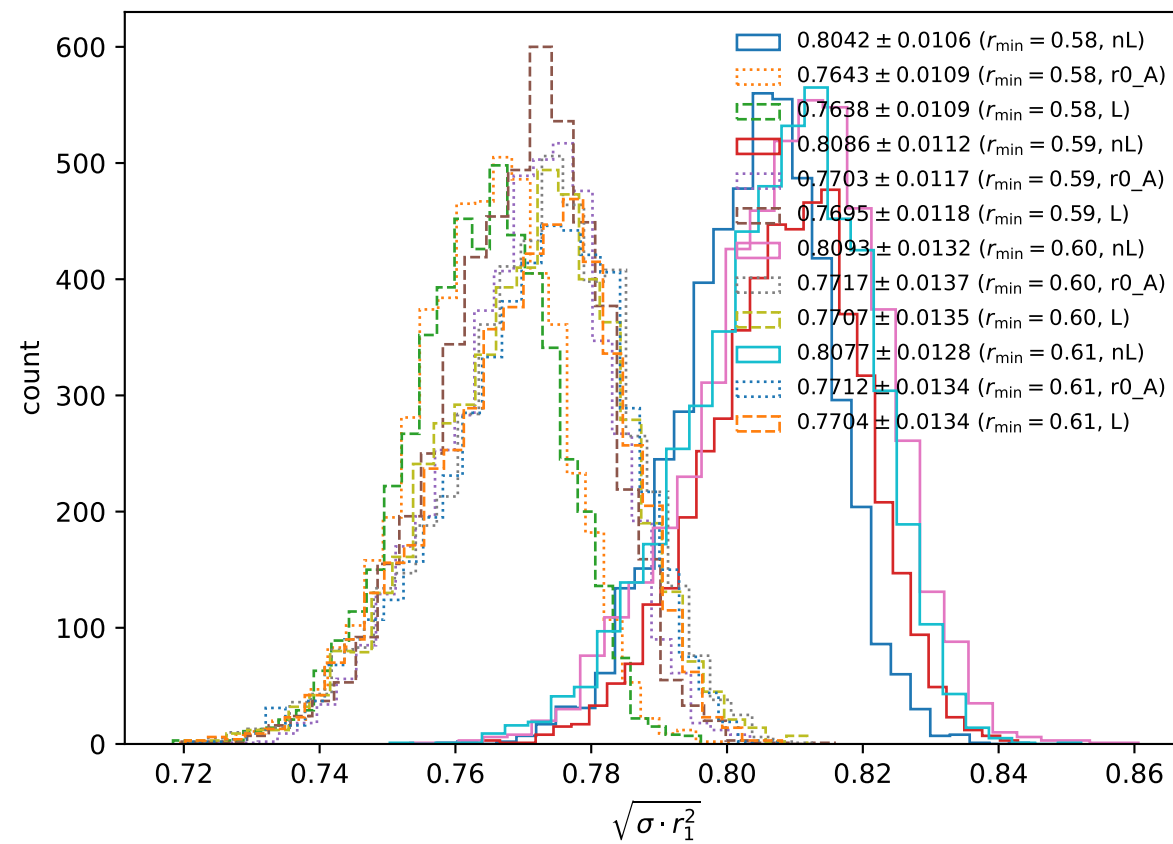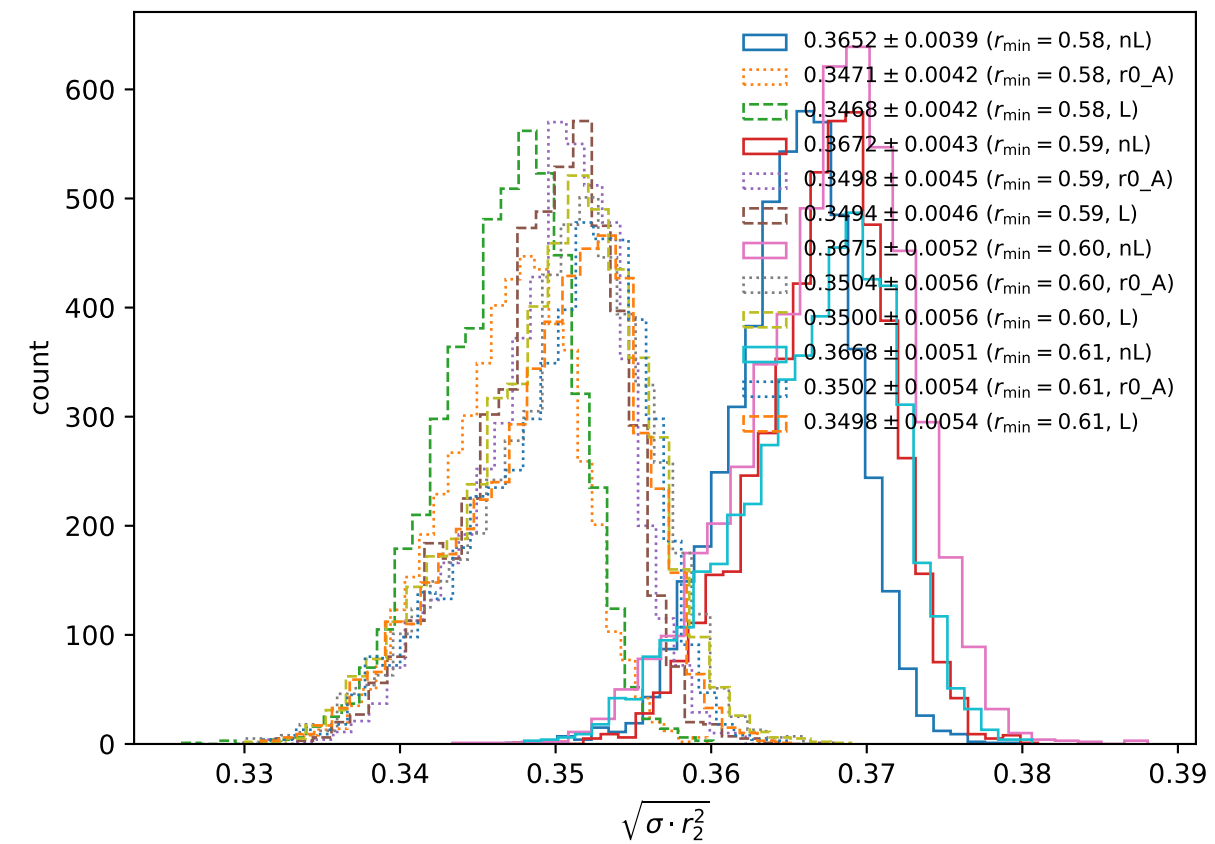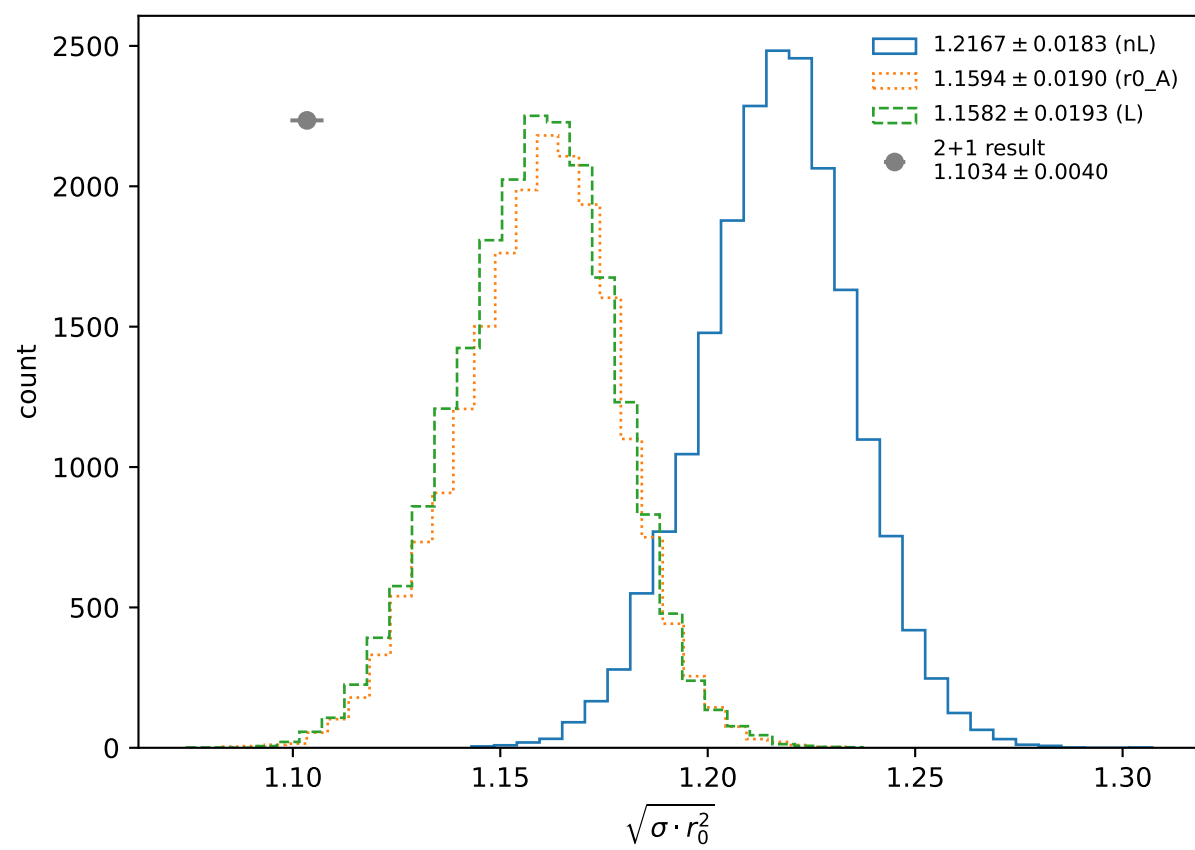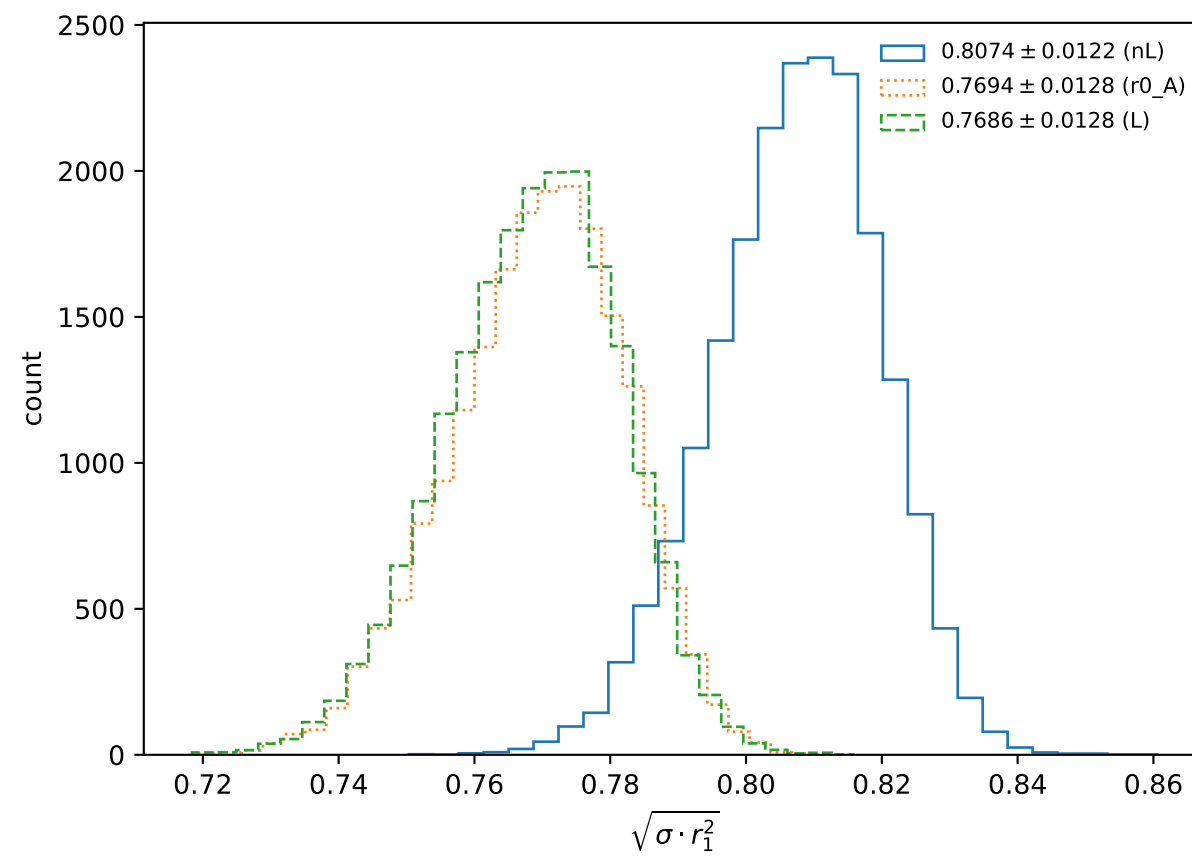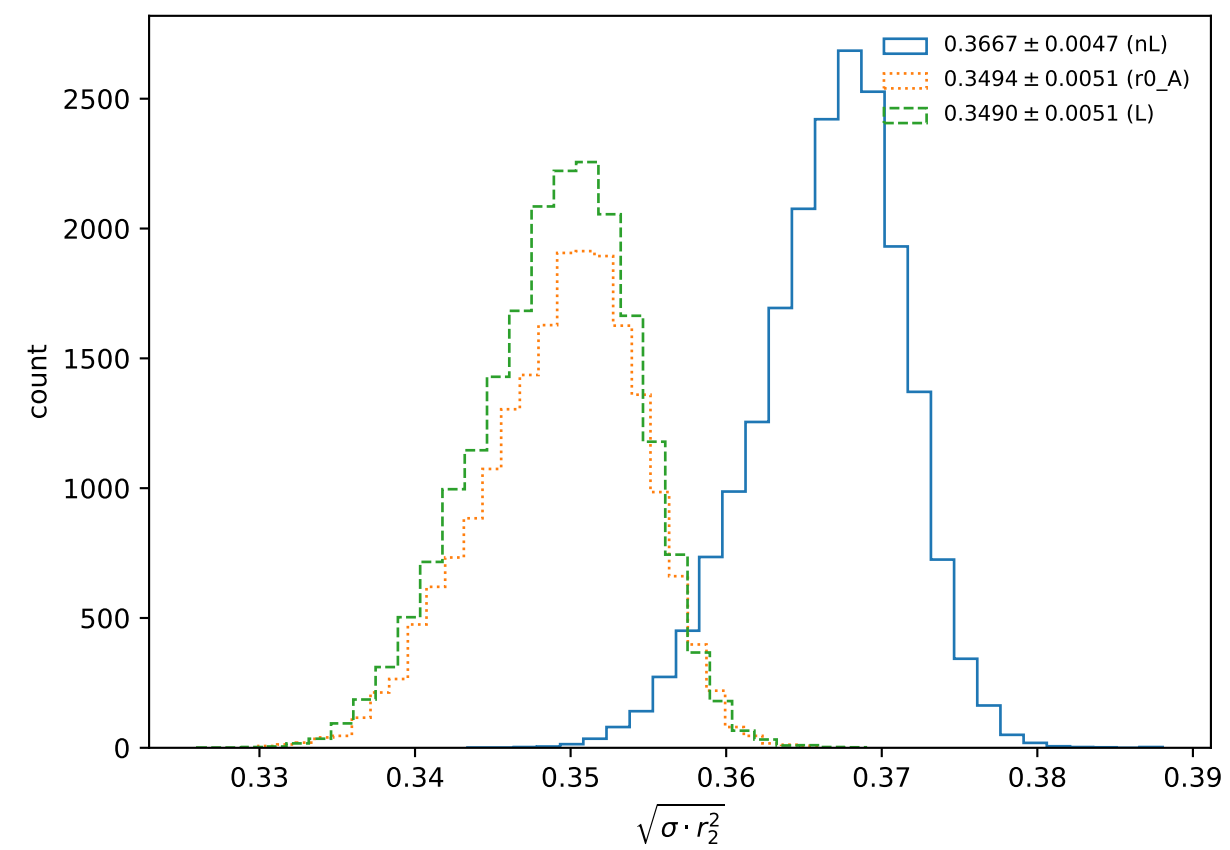



sm1 - method 2 - 5000 resamples - l96192f211b672m0008m022m260

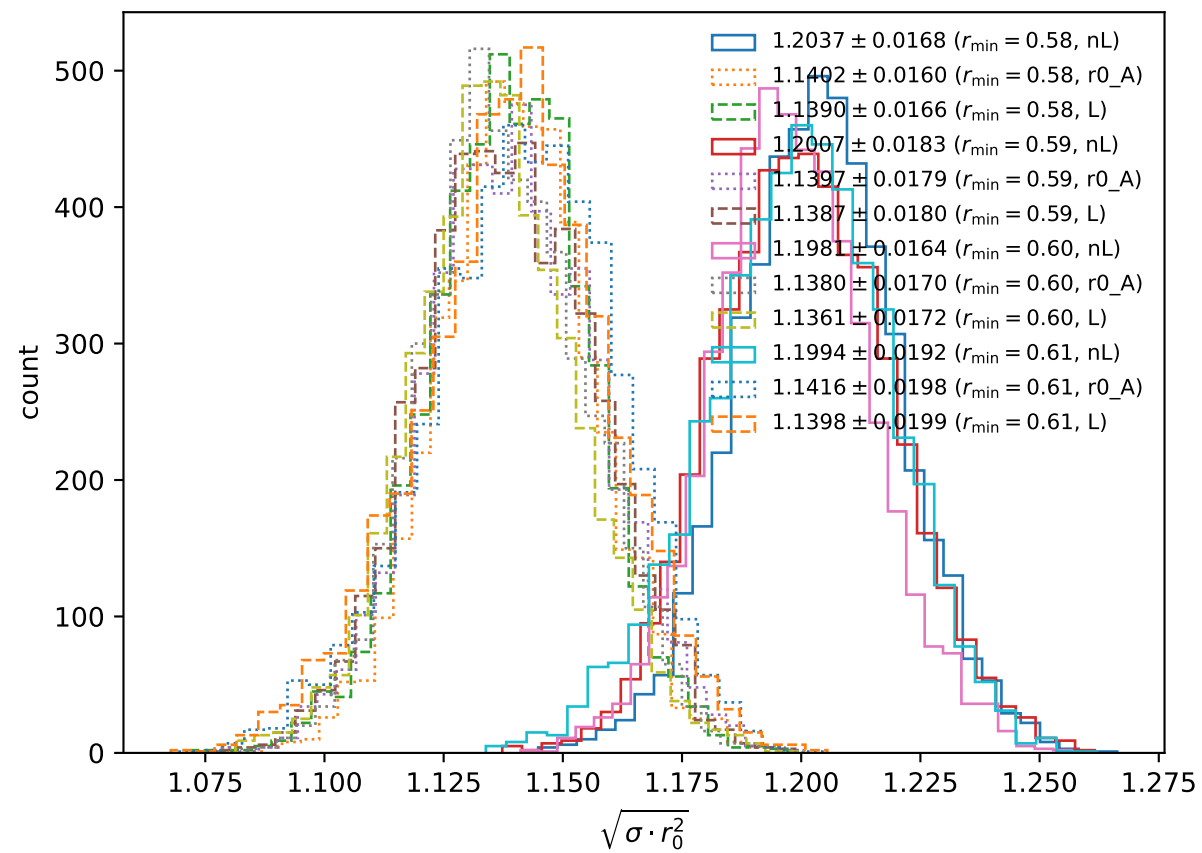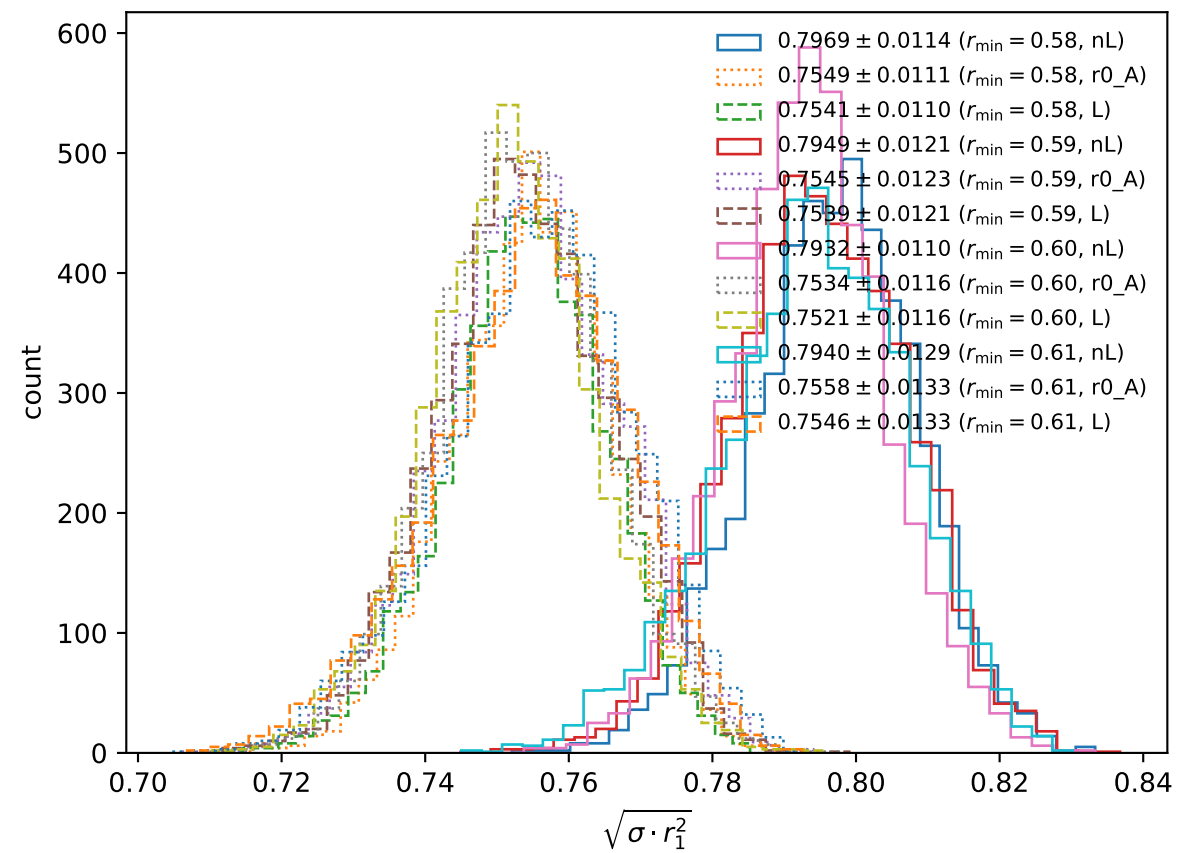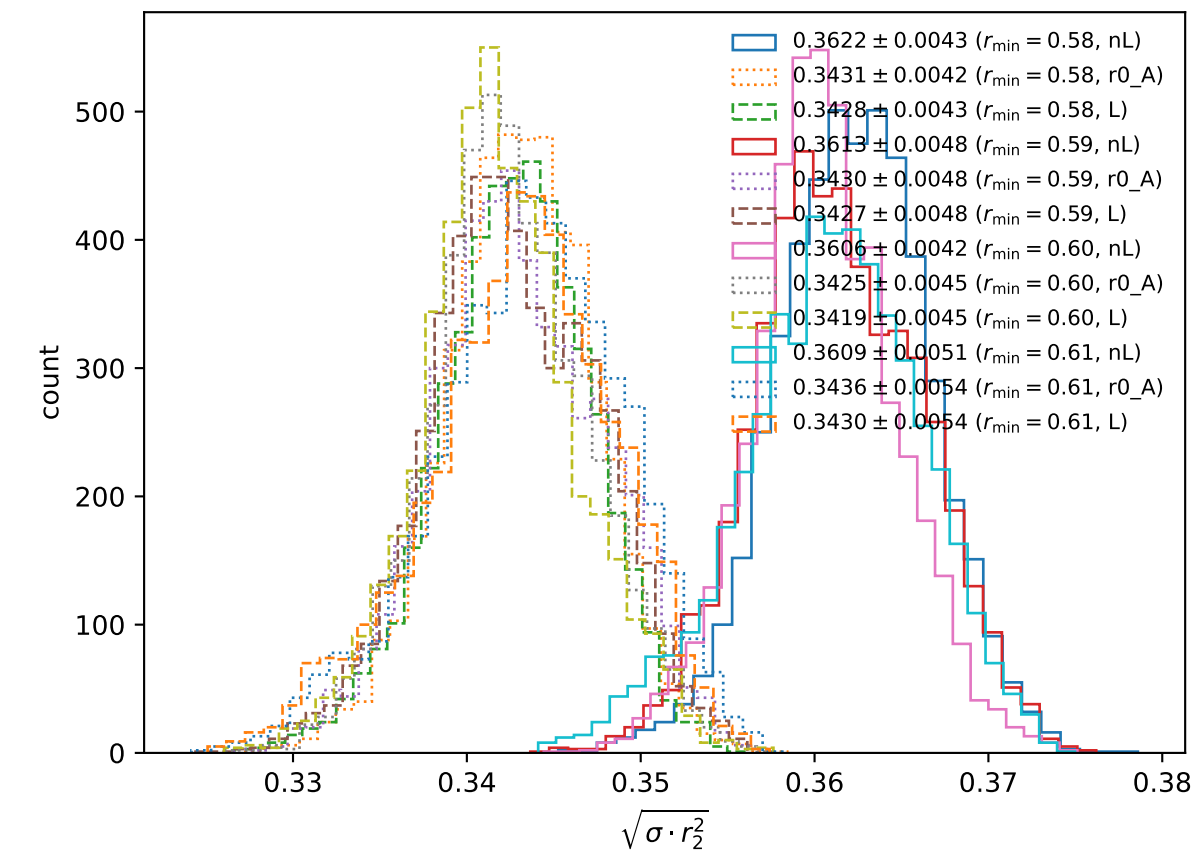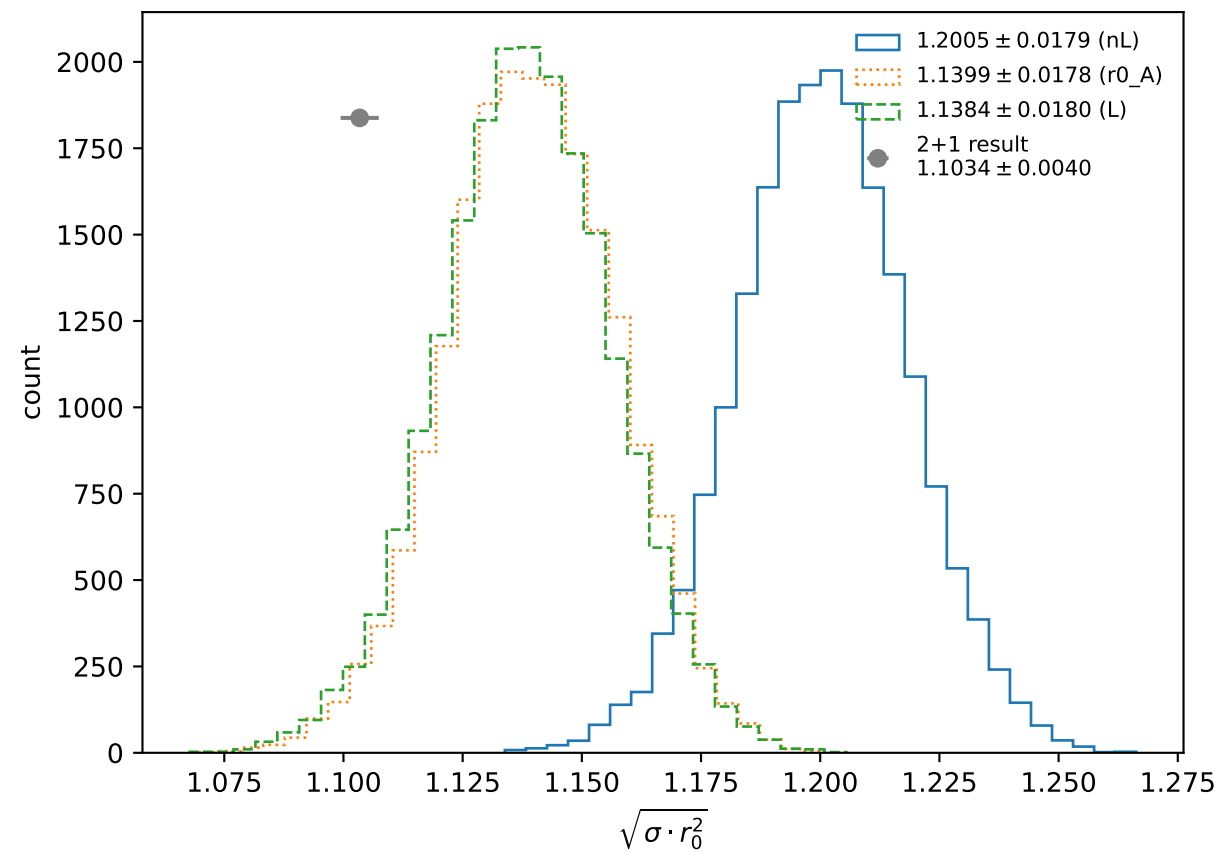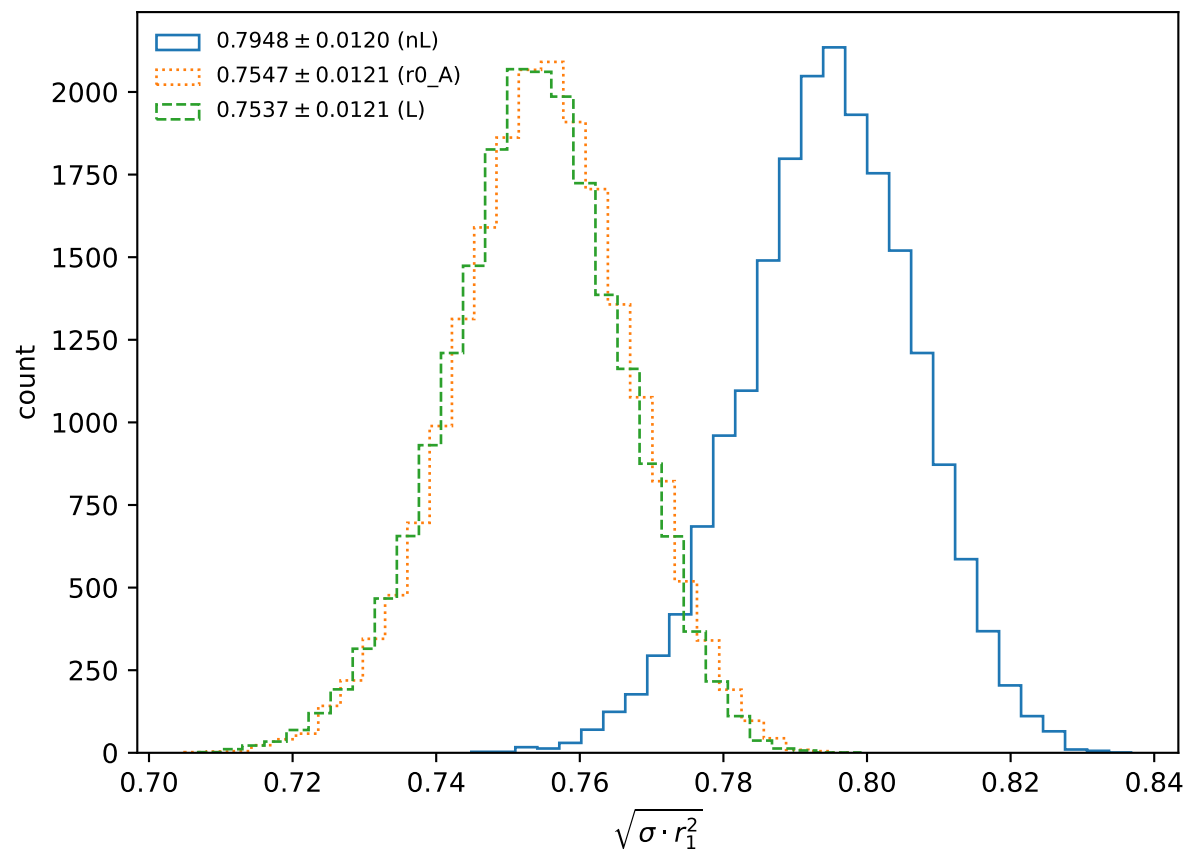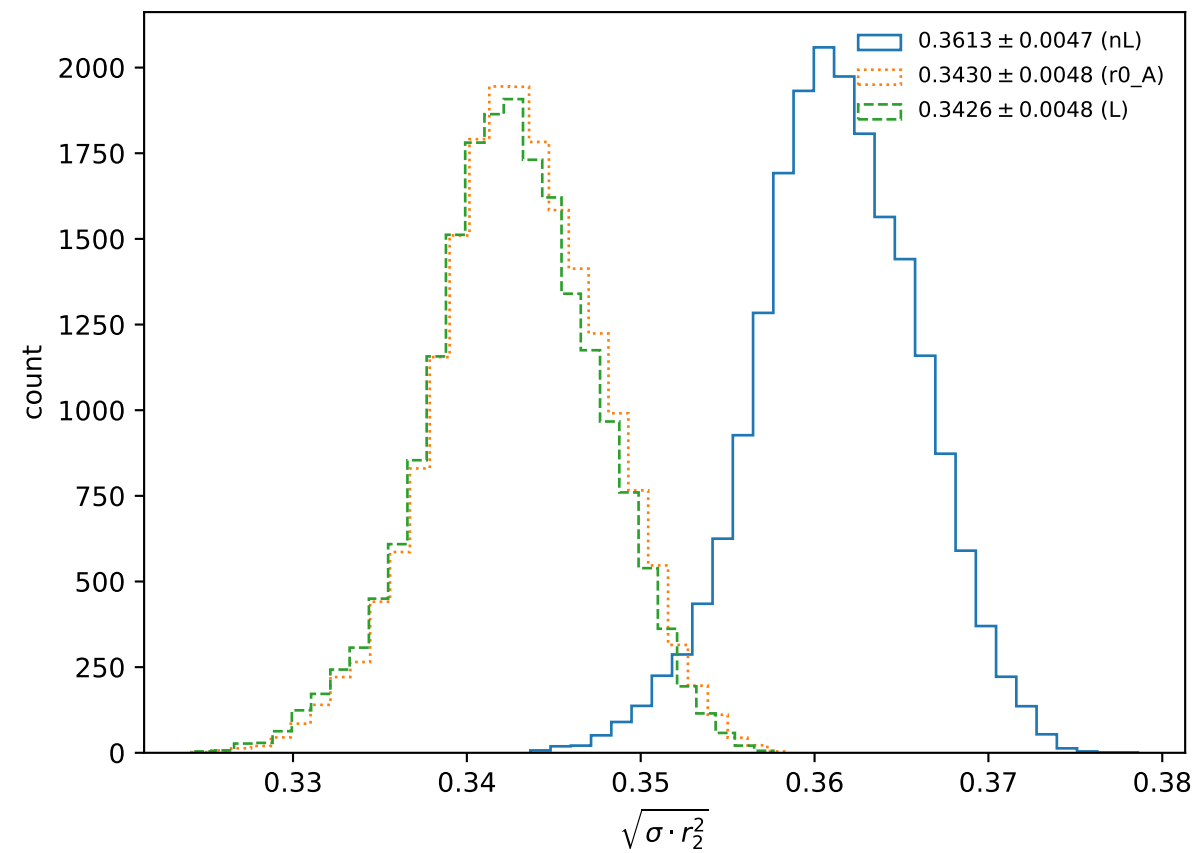

sm1 - method 2 - 5000 resamples - l64192f211b700m00316m0158m188

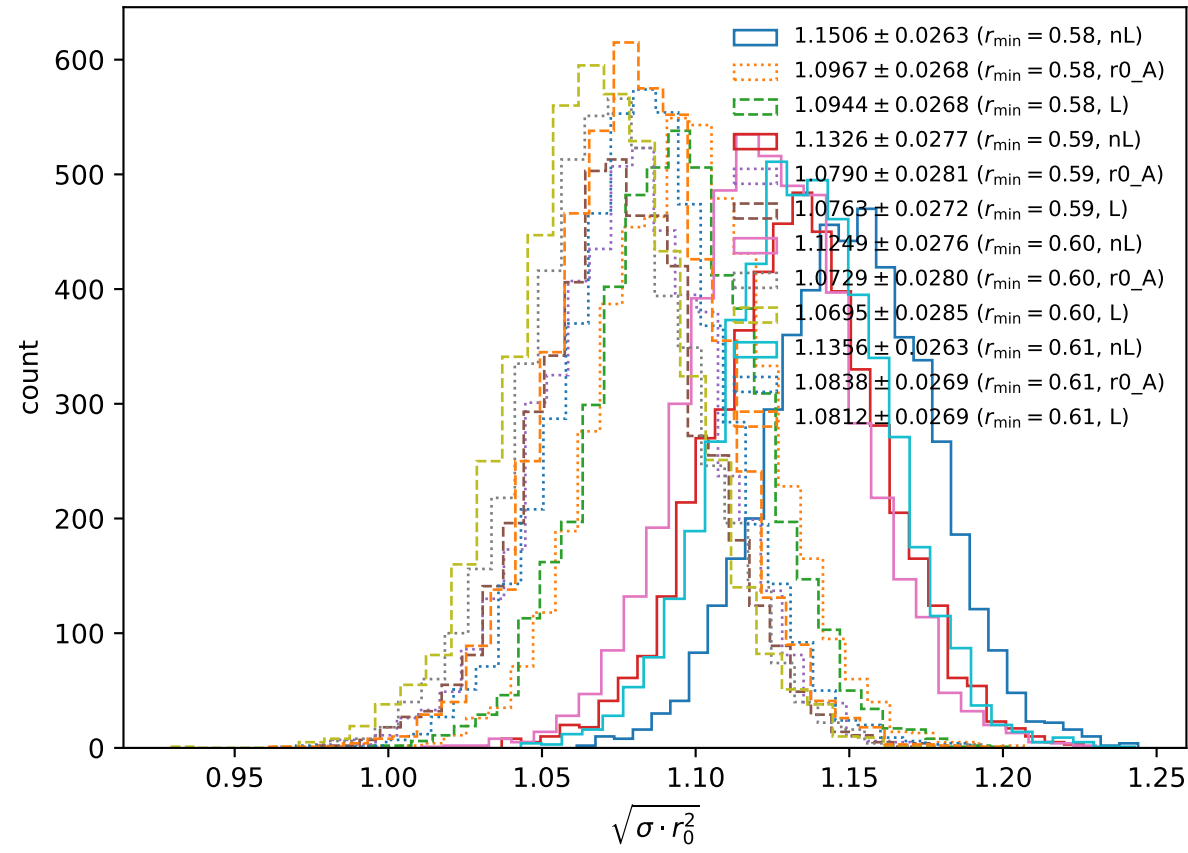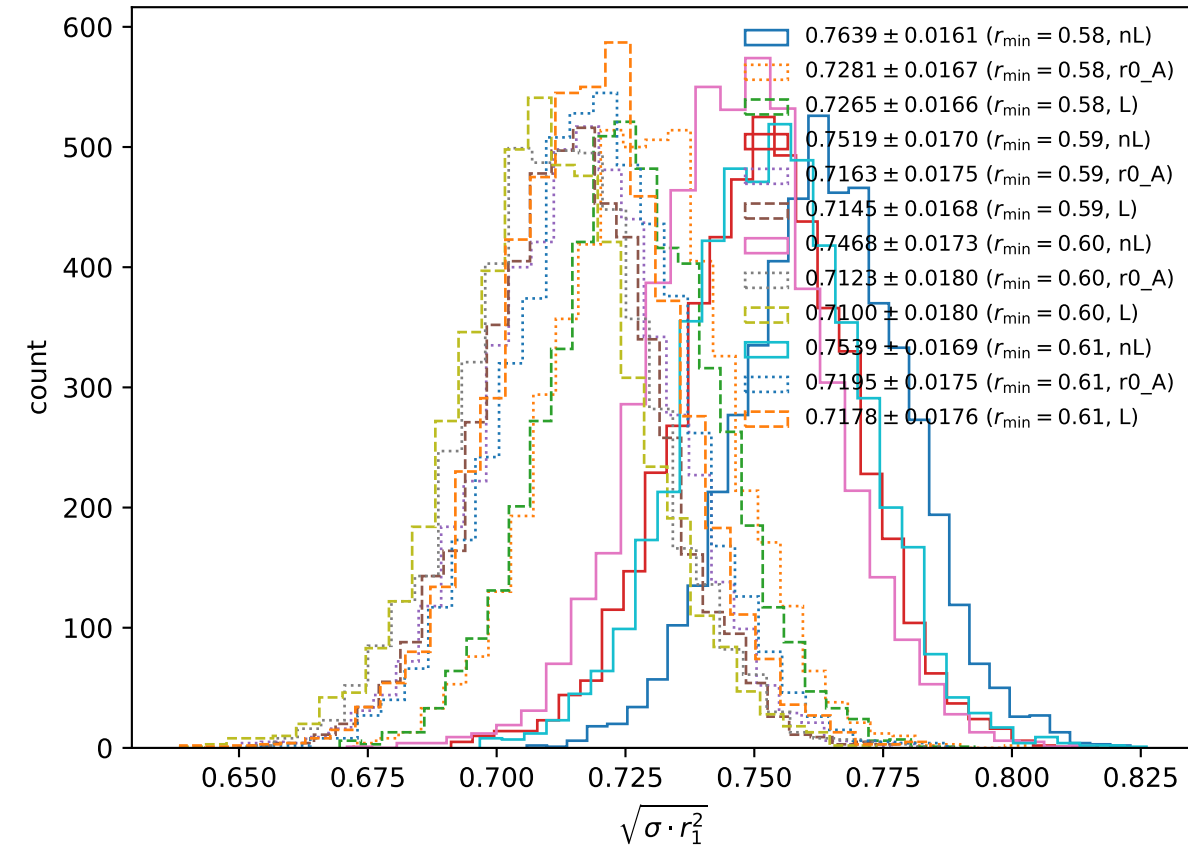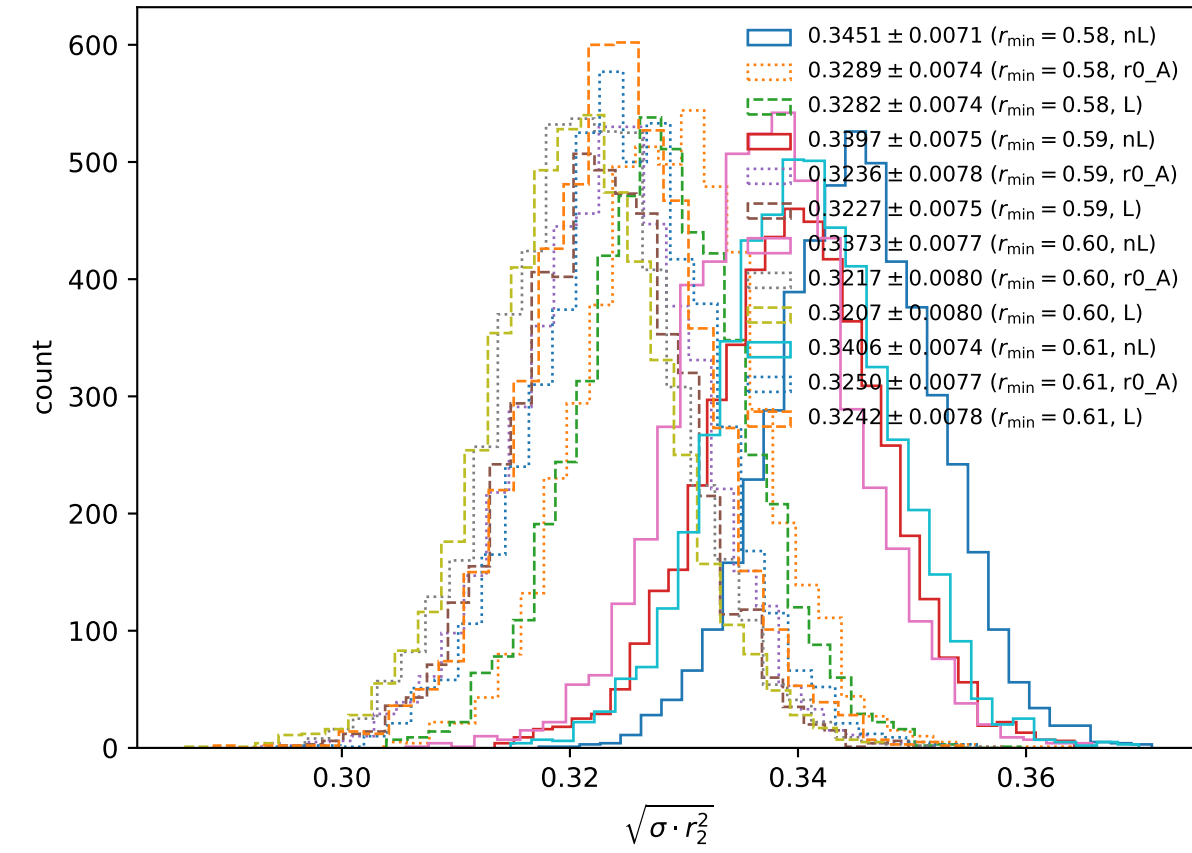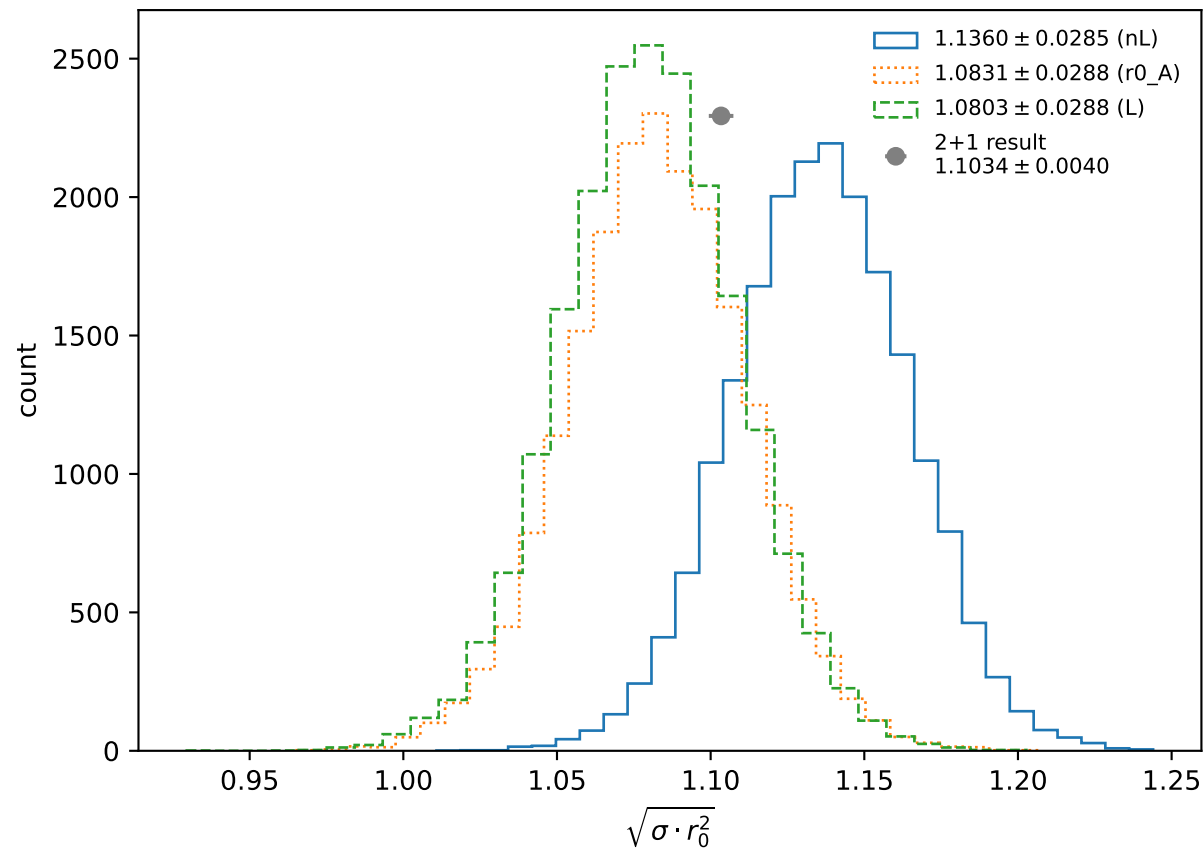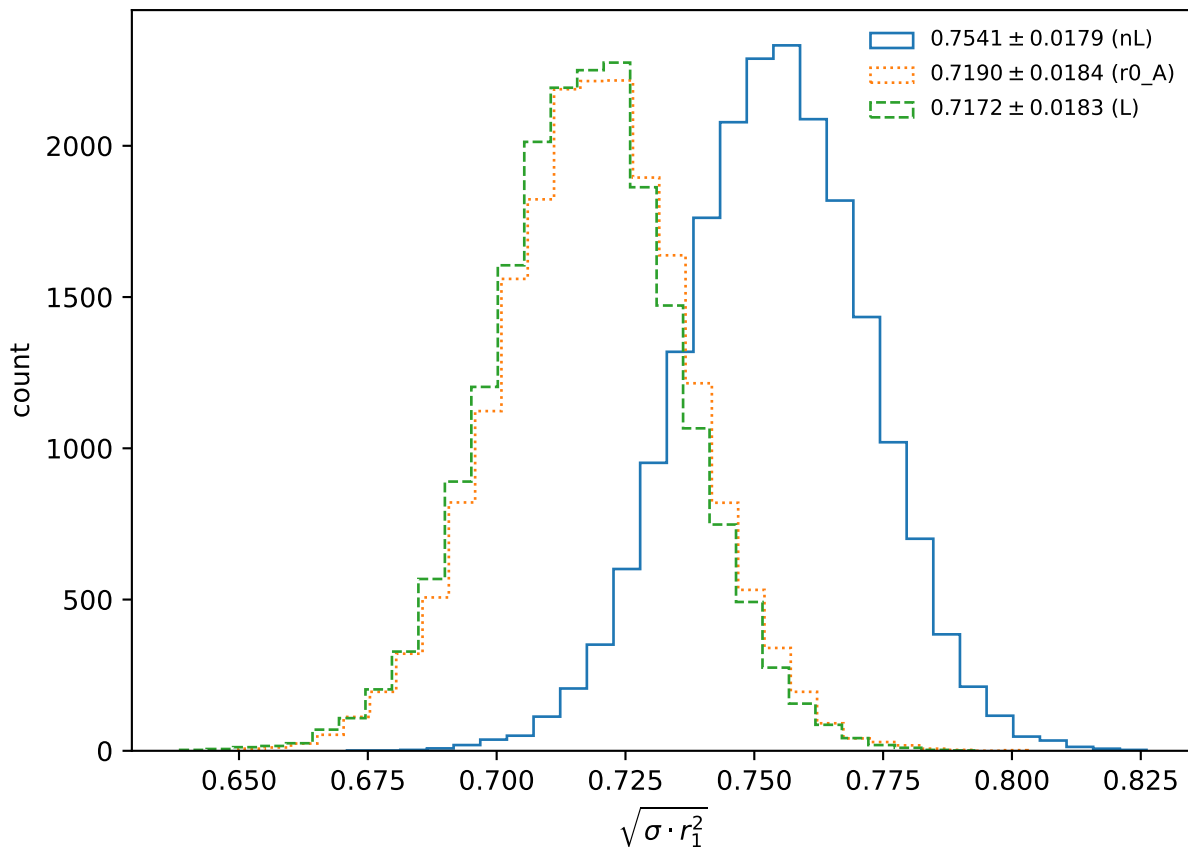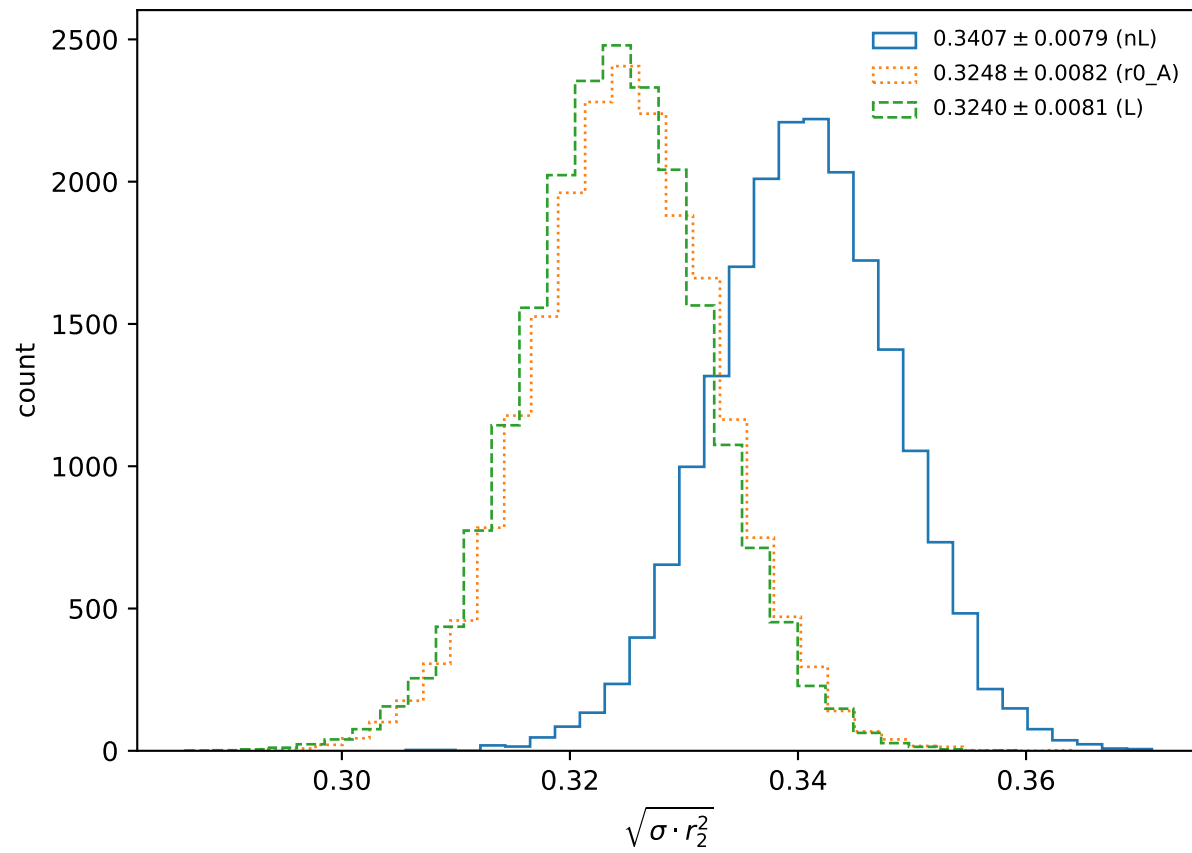

sm1 - method 2 - 5000 resamples - l144288f211b700m000569m01555m1827

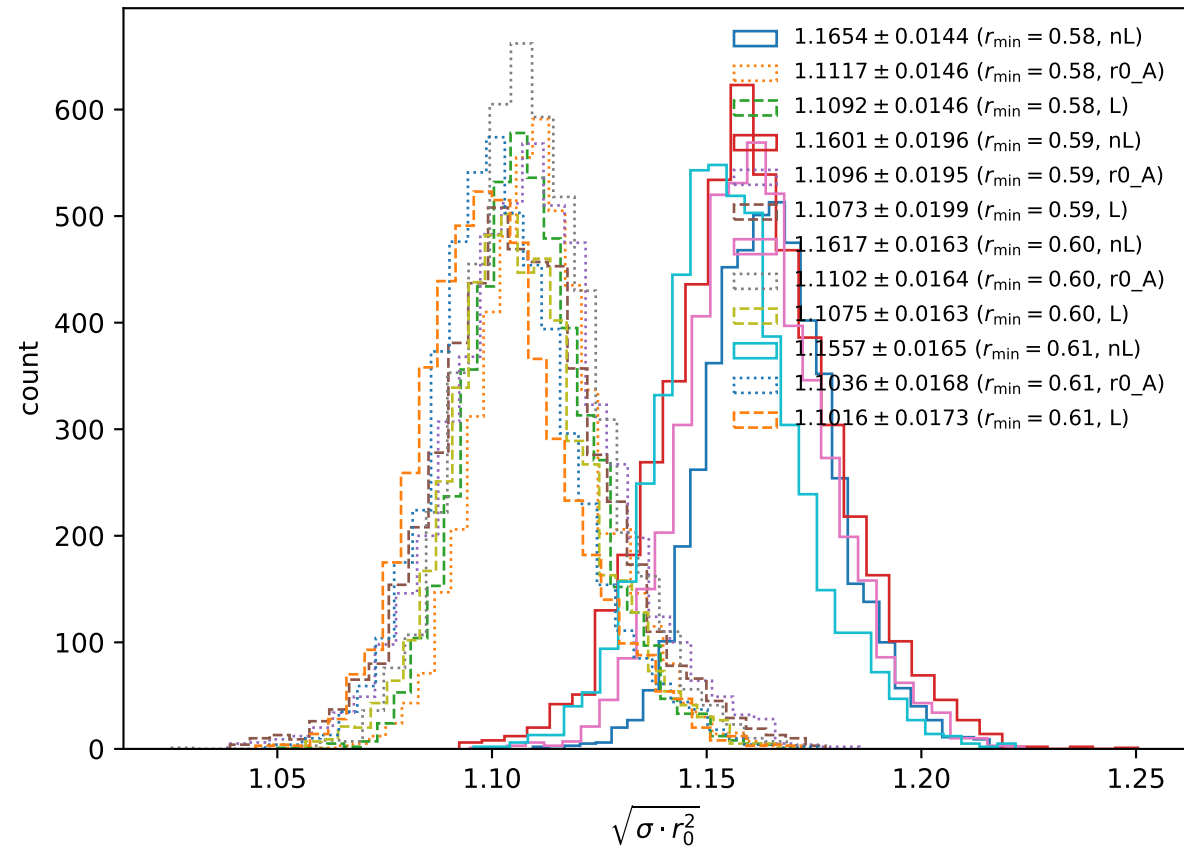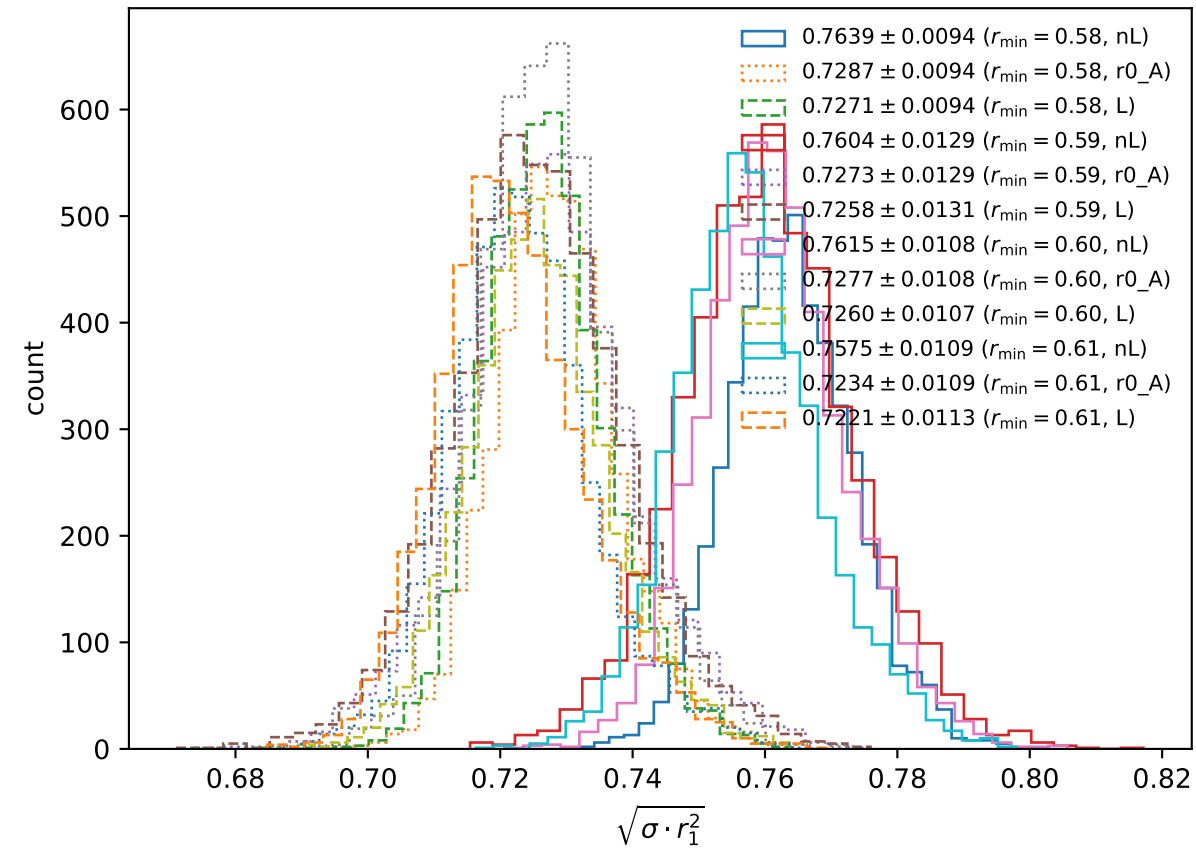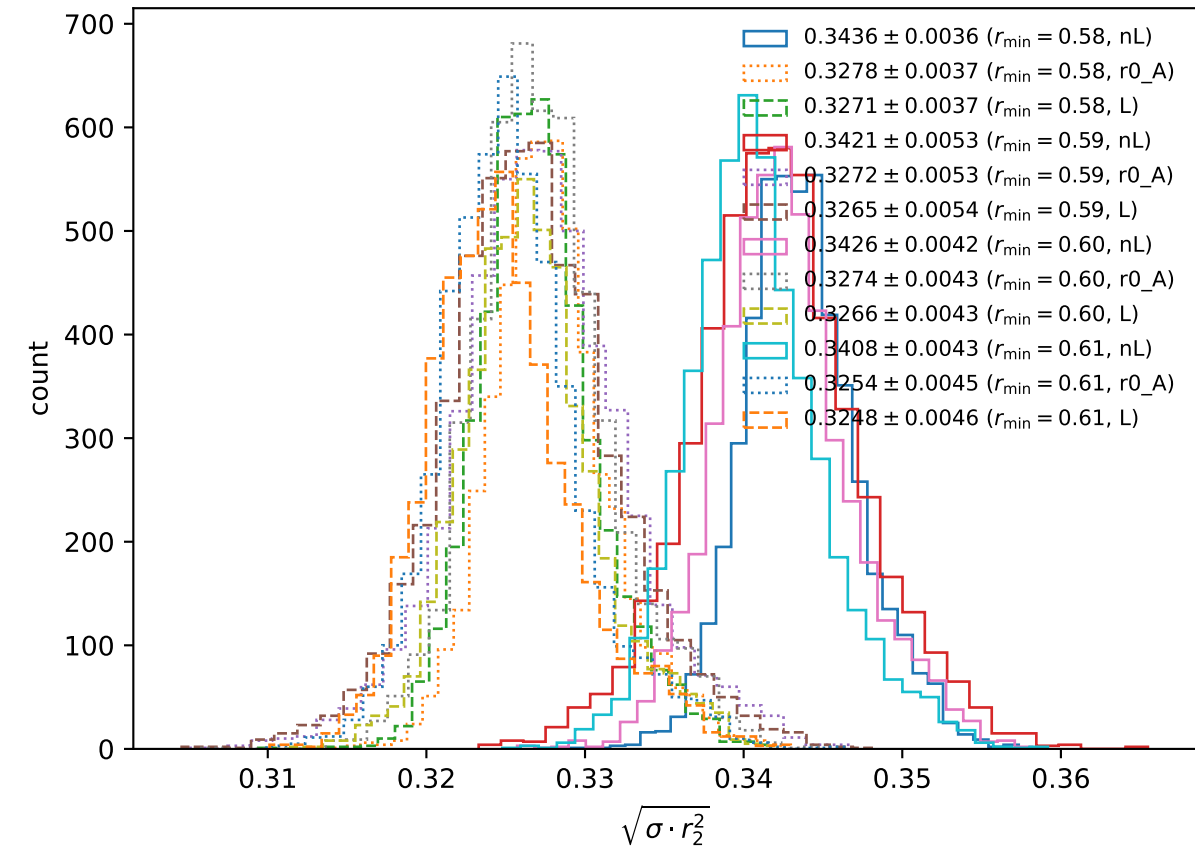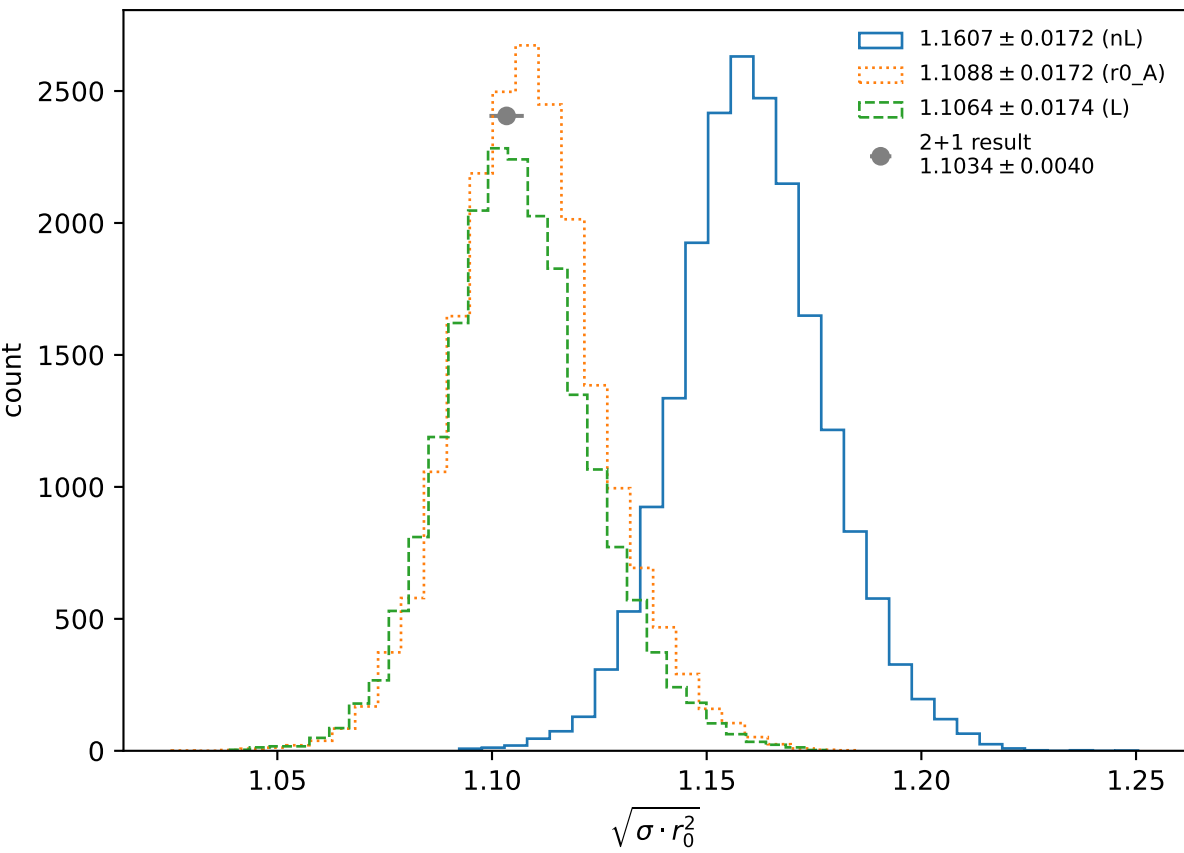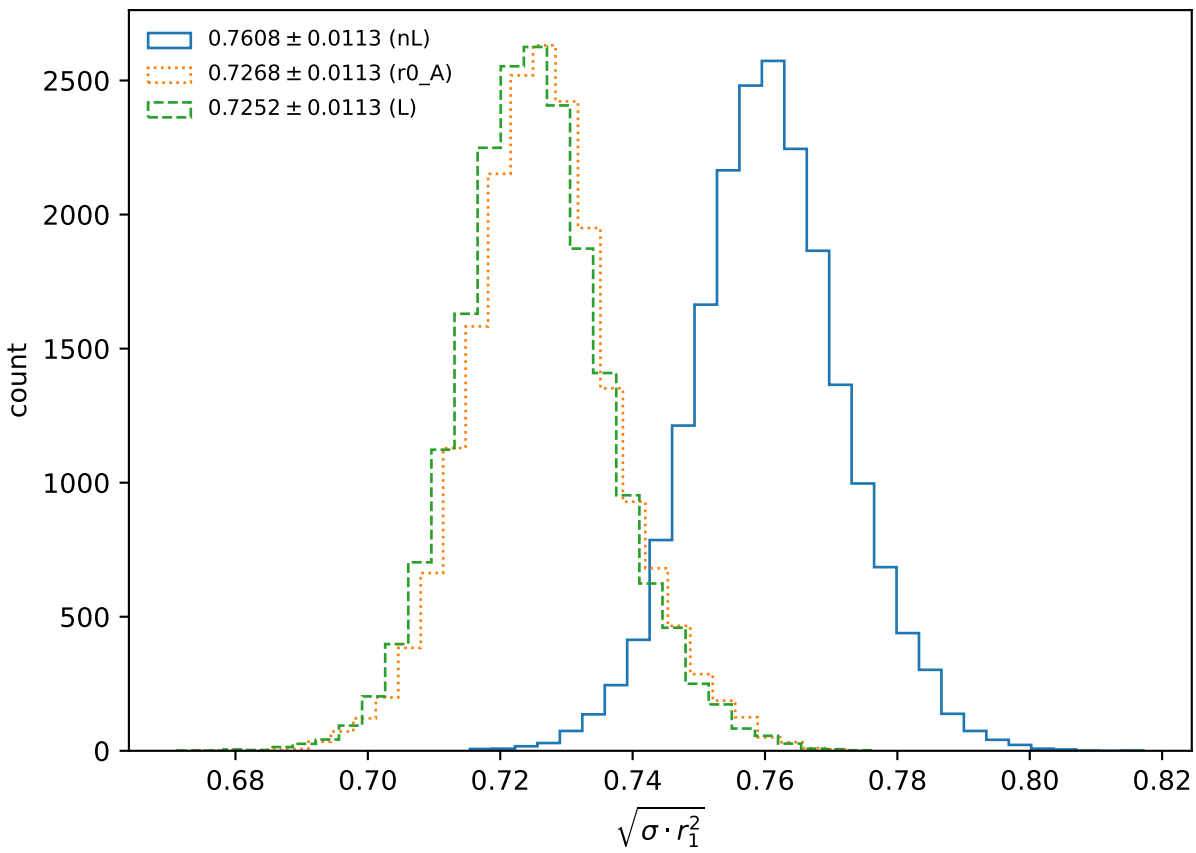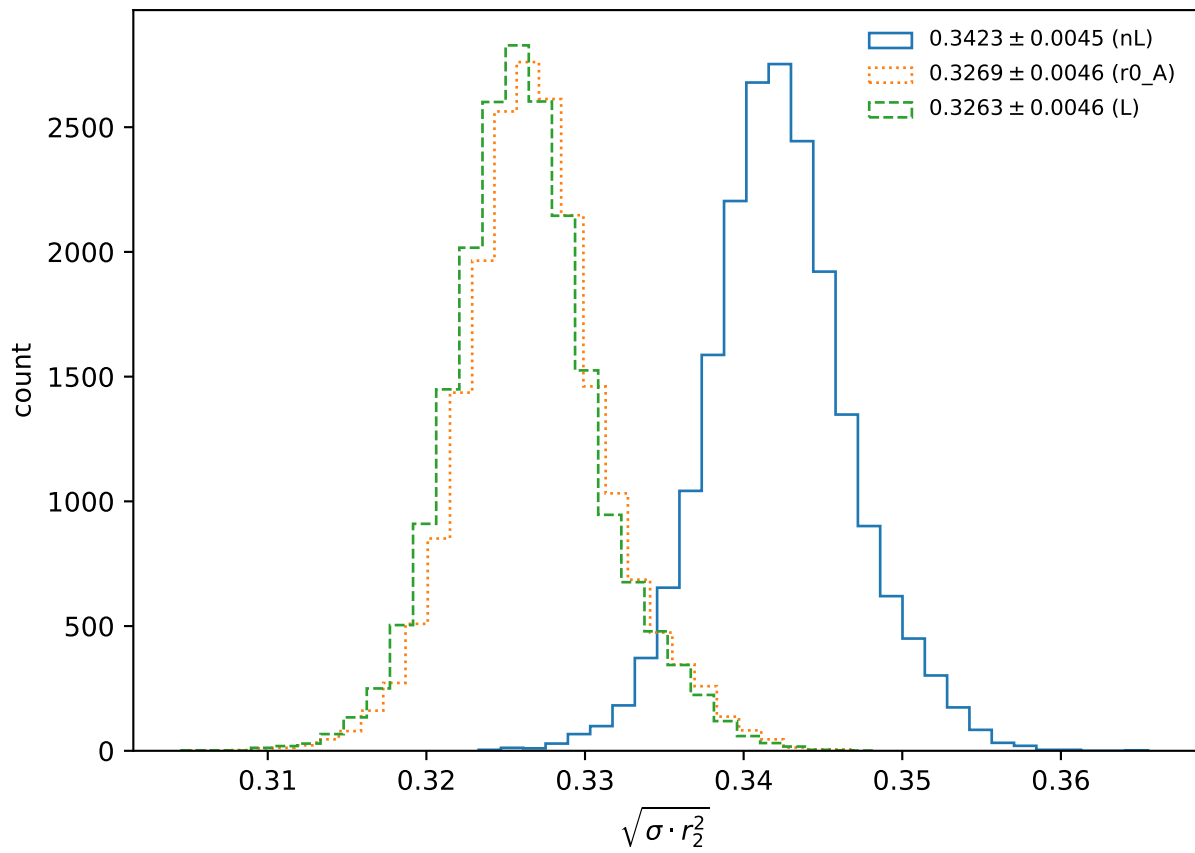

sm1 - method 2 - 5000 resamples - l96288f211b728m00223m01115m1316

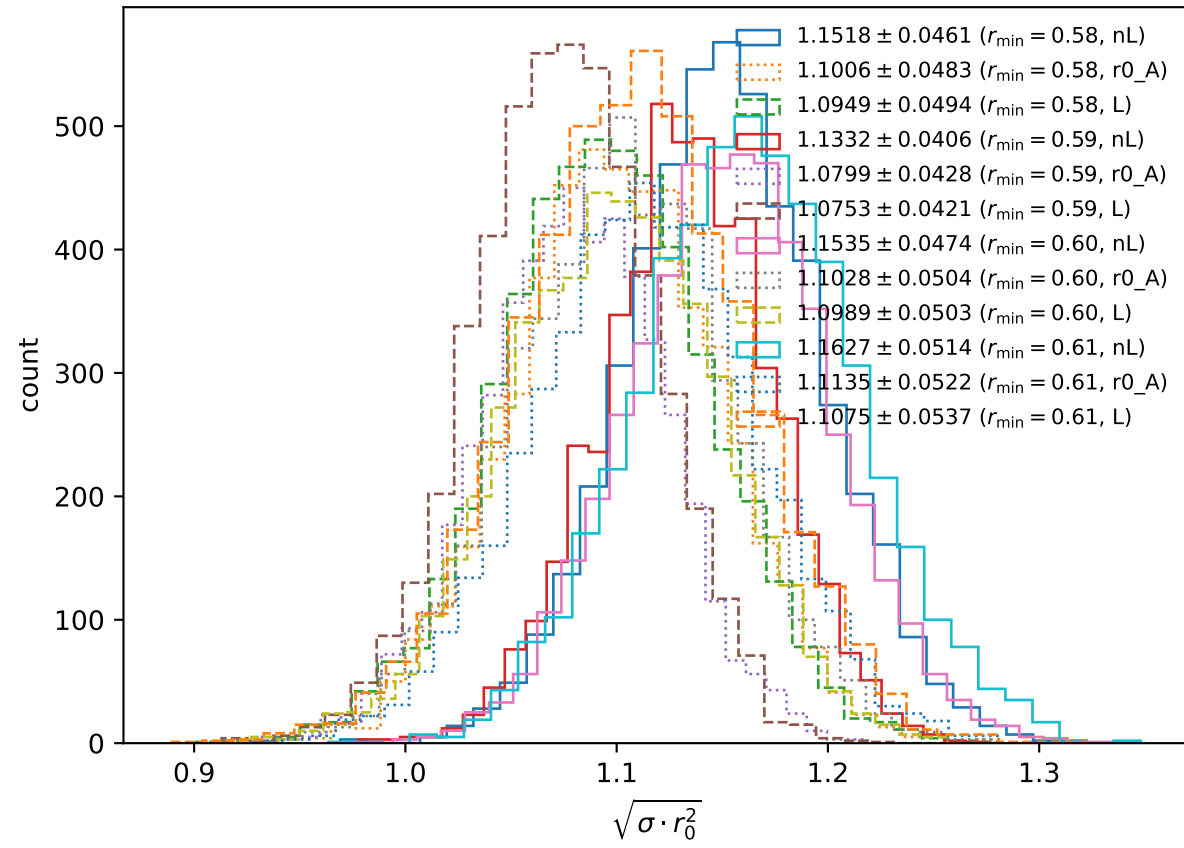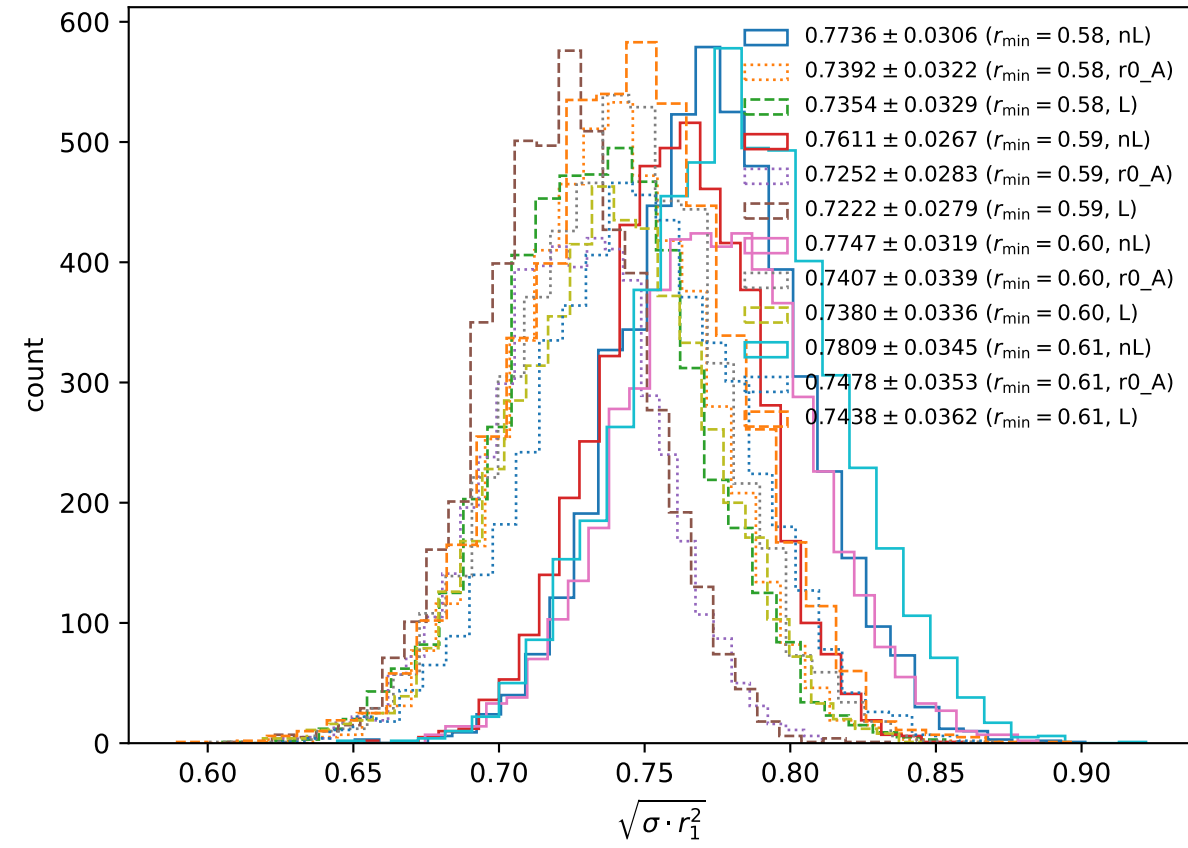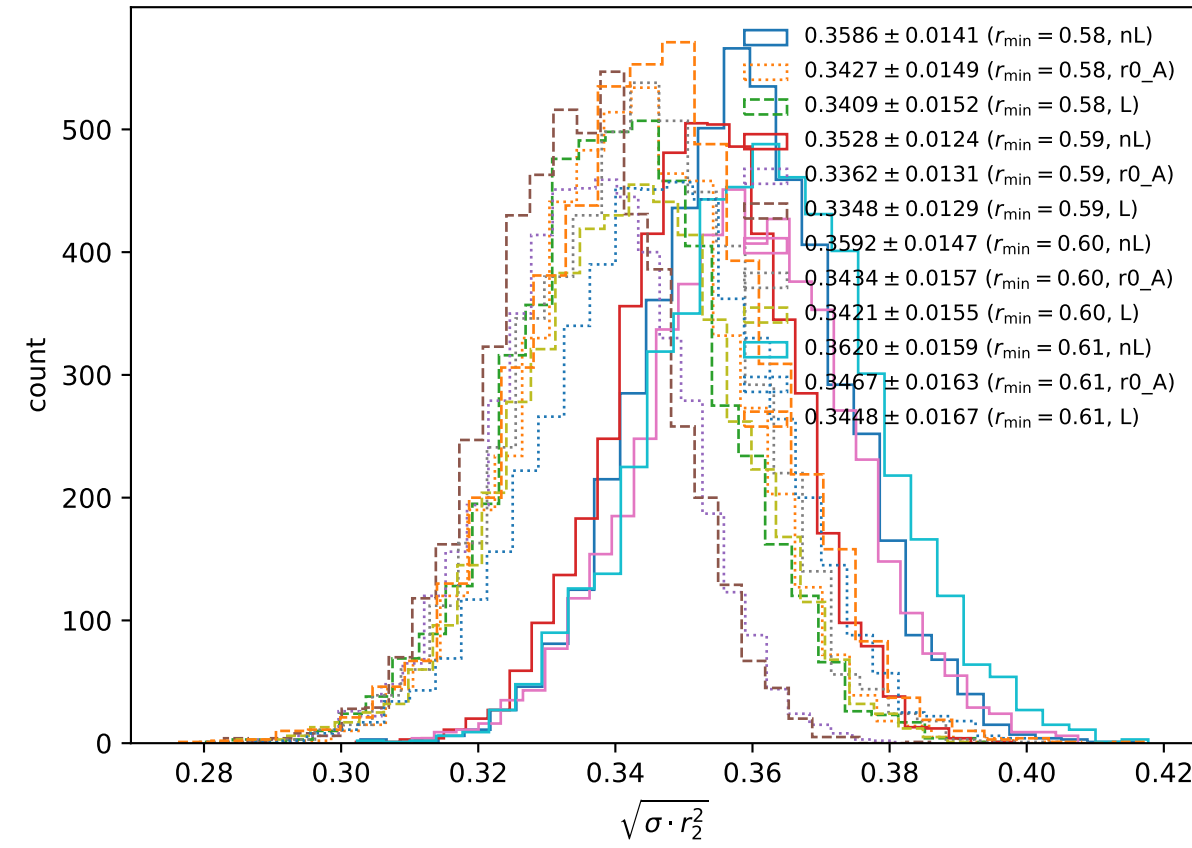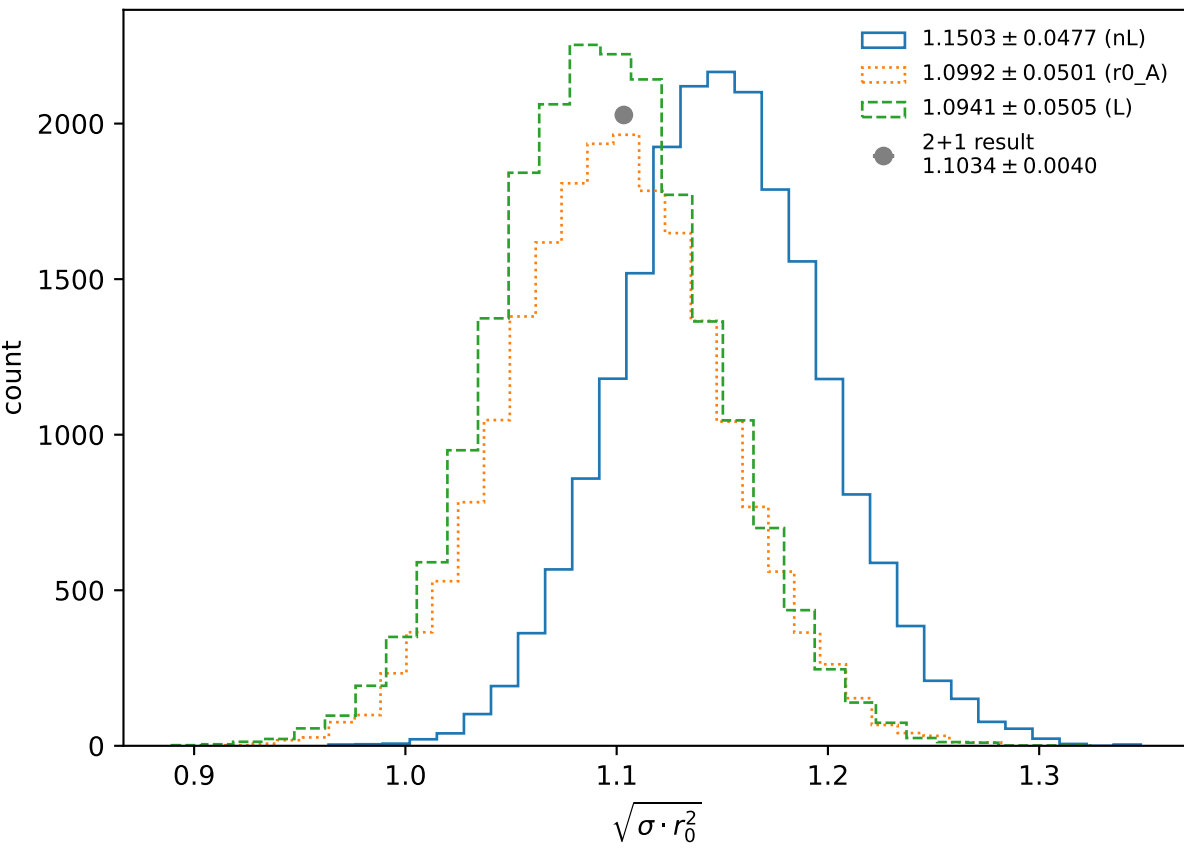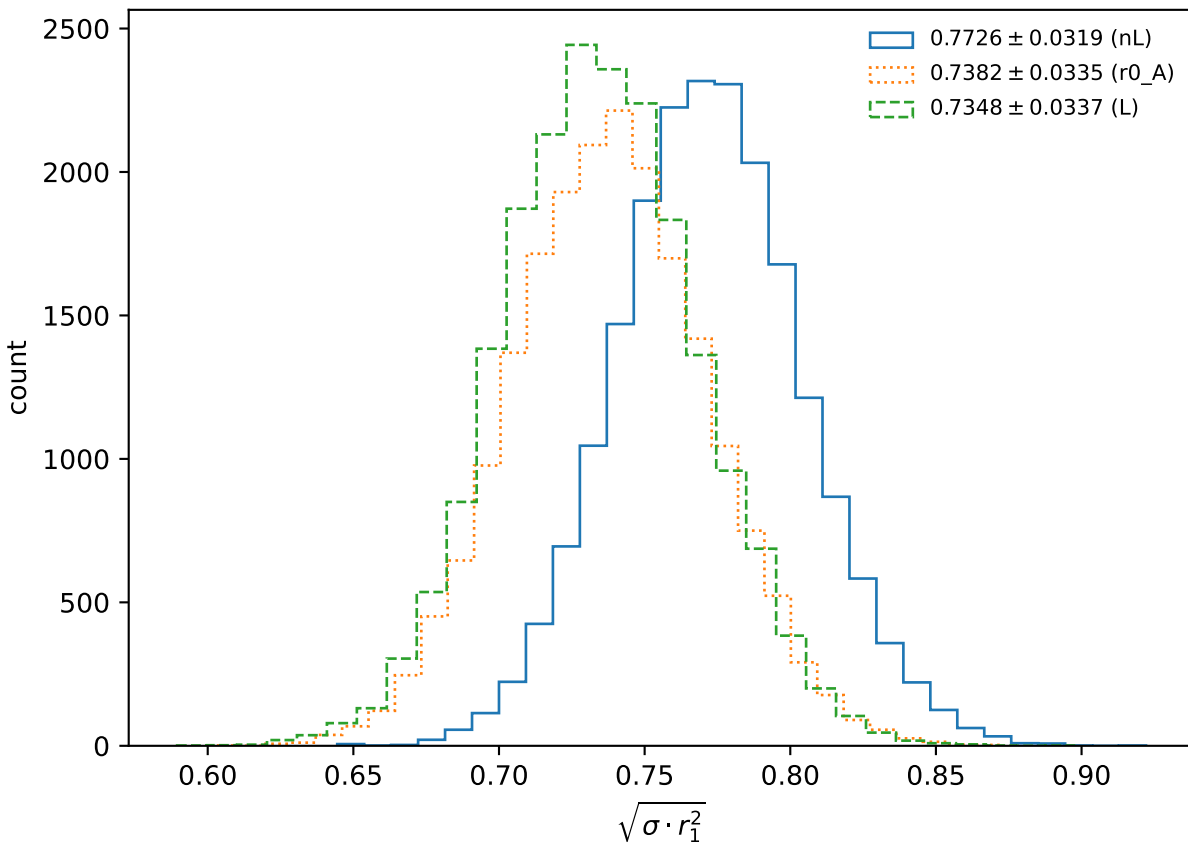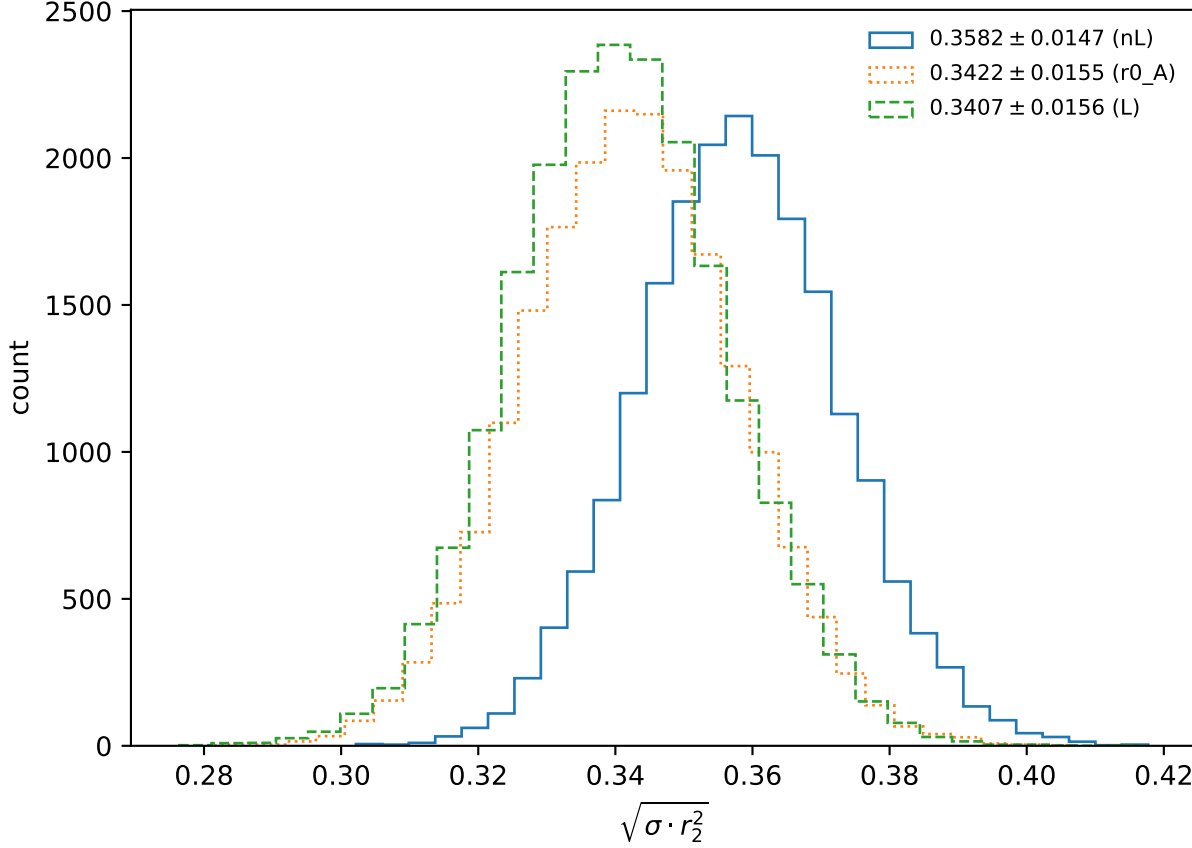

Supplement: Supplementary file 1 [file sigma_r_sq_sm1_method_2_5000_resamples.pdf]
